# Supplementary material for: Failure detection for transport processes on networks
Source: arXiv:2311.02624 source file (2026-05-24)
Supplement: Supplementary file 1 [file SI.tex]

\documentclass[article,
%superscriptaddress,
%groupedaddress,
%unsortedaddress,
%runinaddress,
%frontmatterverbose, 
%preprint,
%preprintnumbers,
%nofootinbib,
%nobibnotes,
%bibnotes,
 amsmath,amssymb,
 aps,
%pra,
%prb,
%rmp,
%prstab,
%prstper,
%floatfix,
]{revtex4-2}
\usepackage[english]{babel}
\usepackage[utf8]{inputenc}
\usepackage[colorinlistoftodos, color=green!40, prependcaption]{todonotes}

%Preamble
\usepackage{amsmath}
\usepackage{mathtools}
\usepackage{breqn}
\usepackage{amsfonts}
\usepackage{braket}
\usepackage{comment}
\usepackage{subcaption}
\usepackage{hyperref}

%To make the title
%\usepackage{authblk}
\begin{document}

\title{Failure detection for transport networks\\ Supplementary Material}
\author{Edoardo Rolando}
\affiliation{Department of Physics Freie Universit\"at Berlin\\}
\author{Armando Bazzani}
\affiliation{Department of Physics and Astronomy Bologna University}
\affiliation{INFN sezione di Bologna\\}

\maketitle

%%%%%%%%%%%%%%%%%%%%%%%%%%%%%%%%%%%%%%%%%%%%%%%%%%%%%%%%%%%%%

%\clearpage
\section{Properties of the covariance matrix in presence of link perturbations}\label{SI:correlation matrix information}

%Eigenvectors of the Covariance matrix
\begin{figure}[h]
    \begin{subfigure}{0.5\textwidth}
        {\centering
        \includegraphics[width=\linewidth]{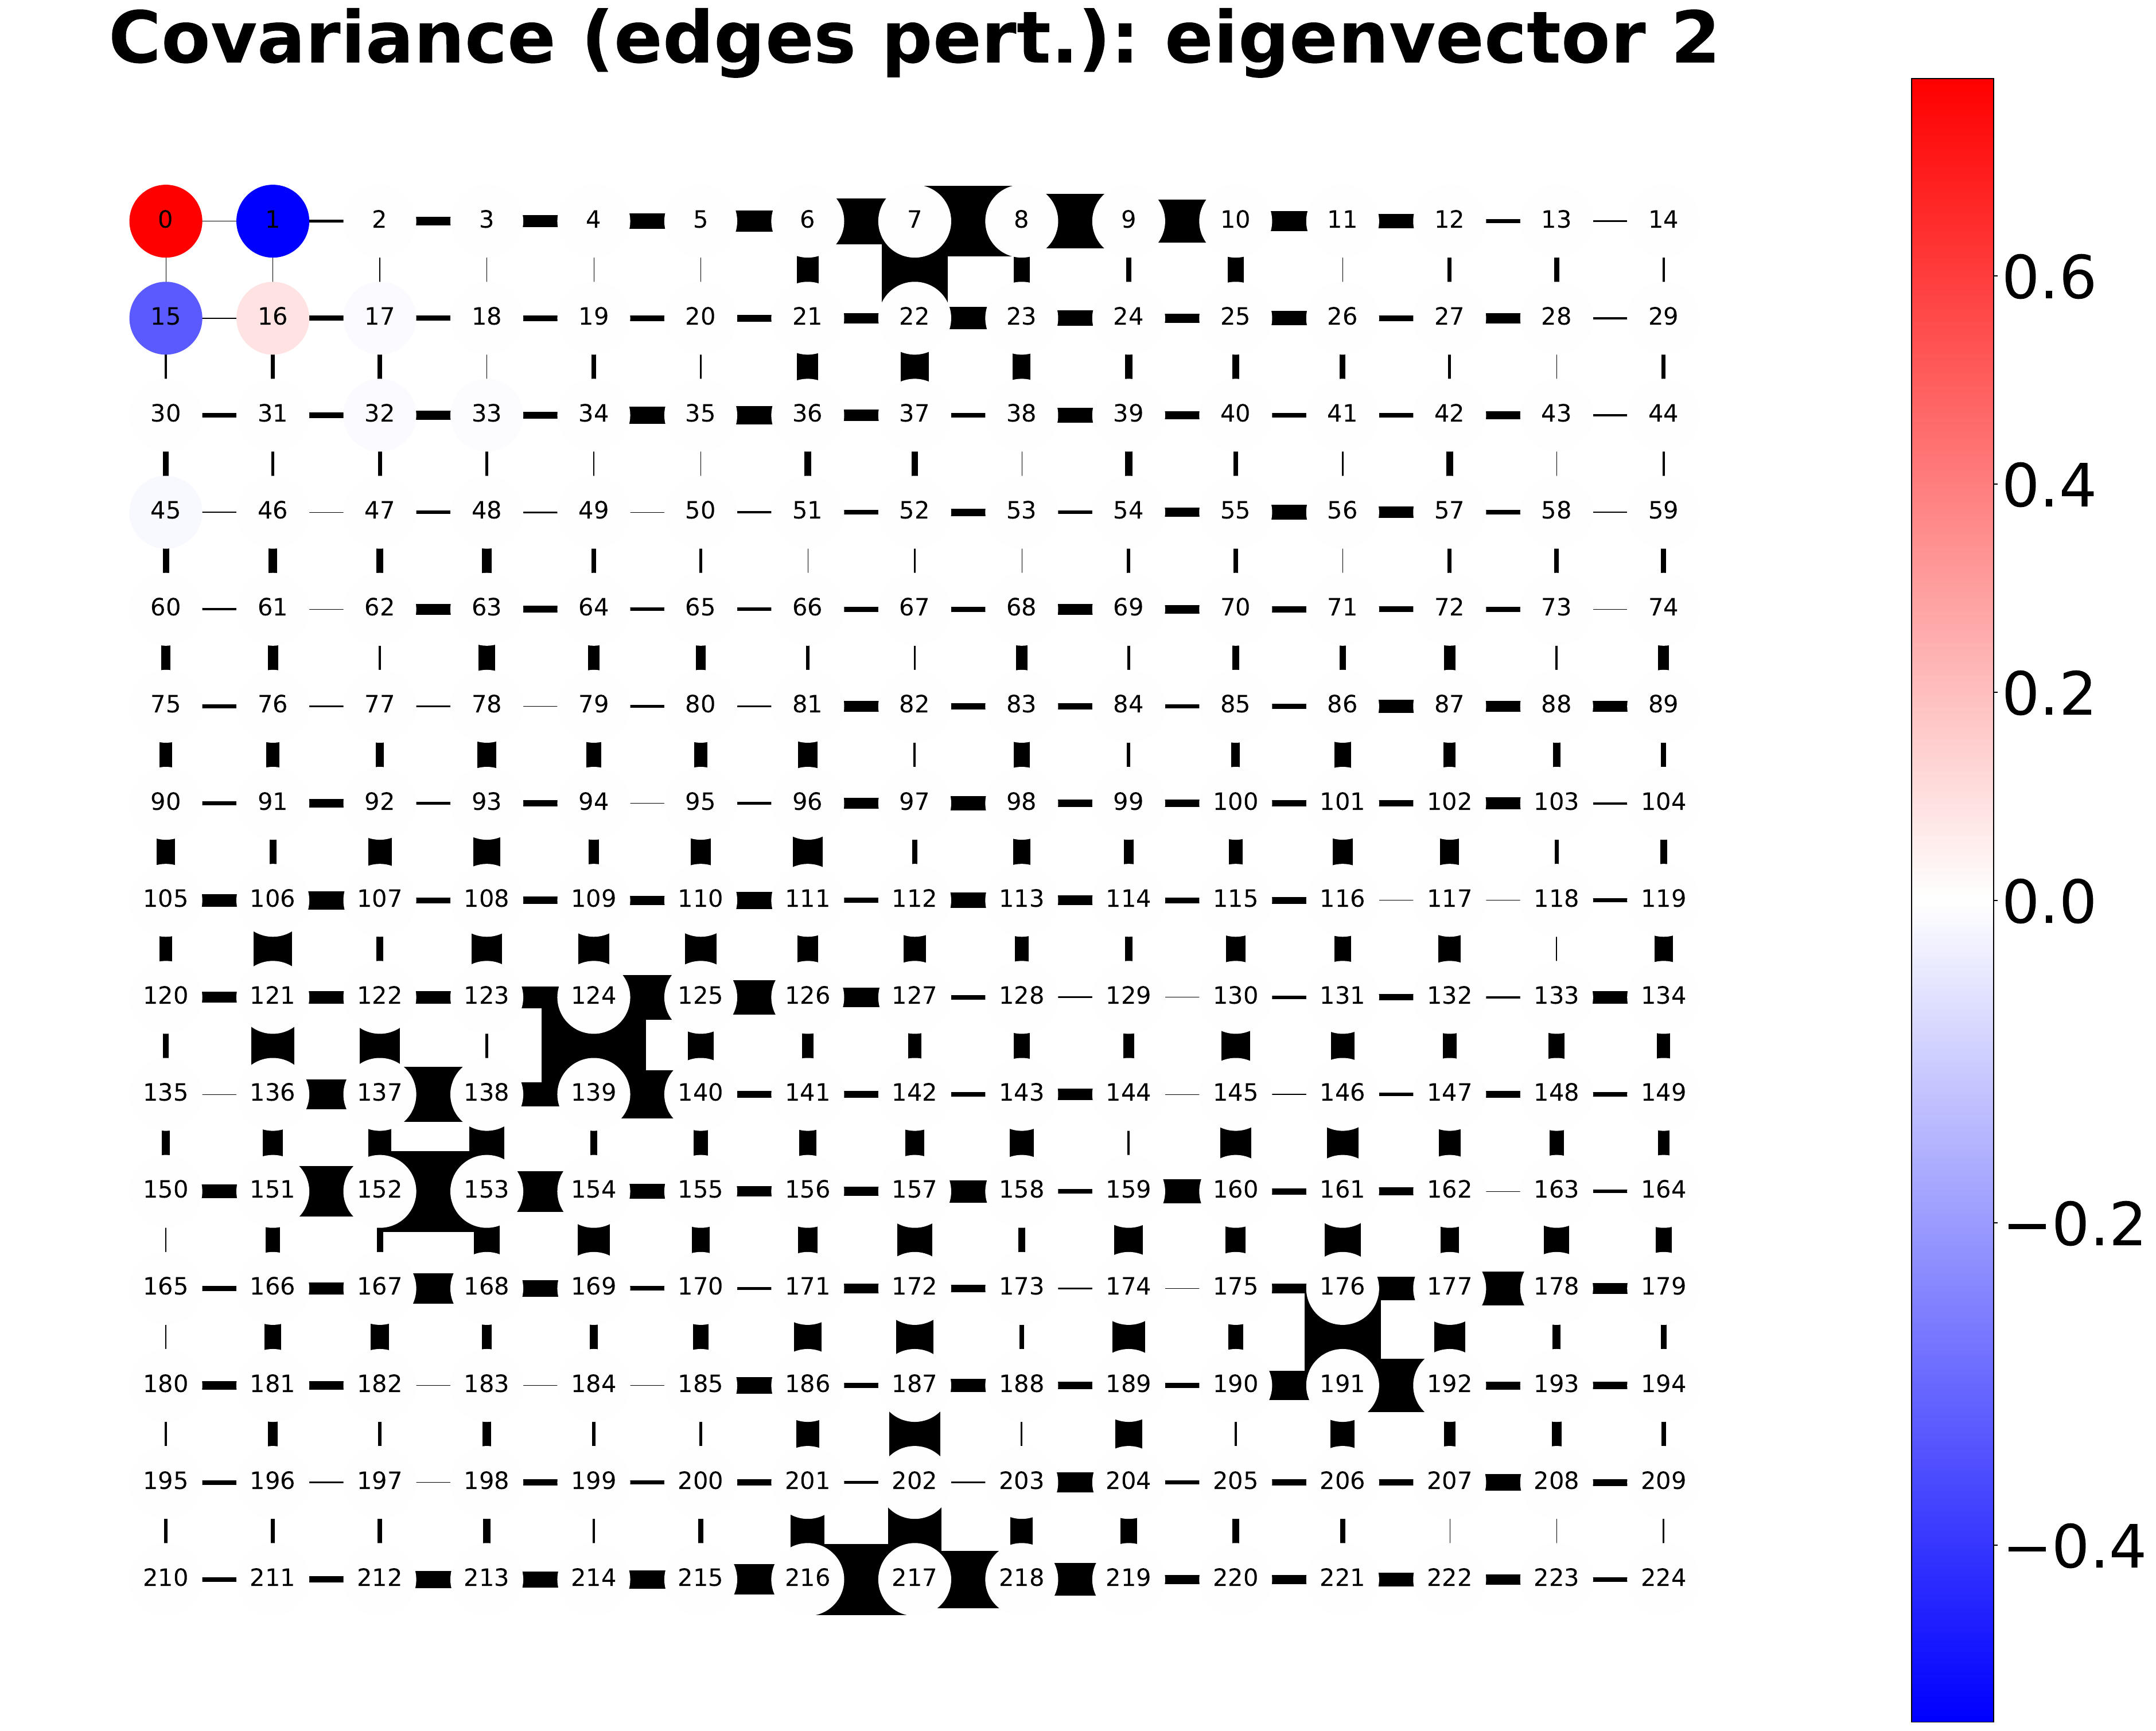}}
    \end{subfigure}\hfill % <-- "\hfill"
    \begin{subfigure}{0.5\textwidth}
        {\centering
        \includegraphics[width=\linewidth]{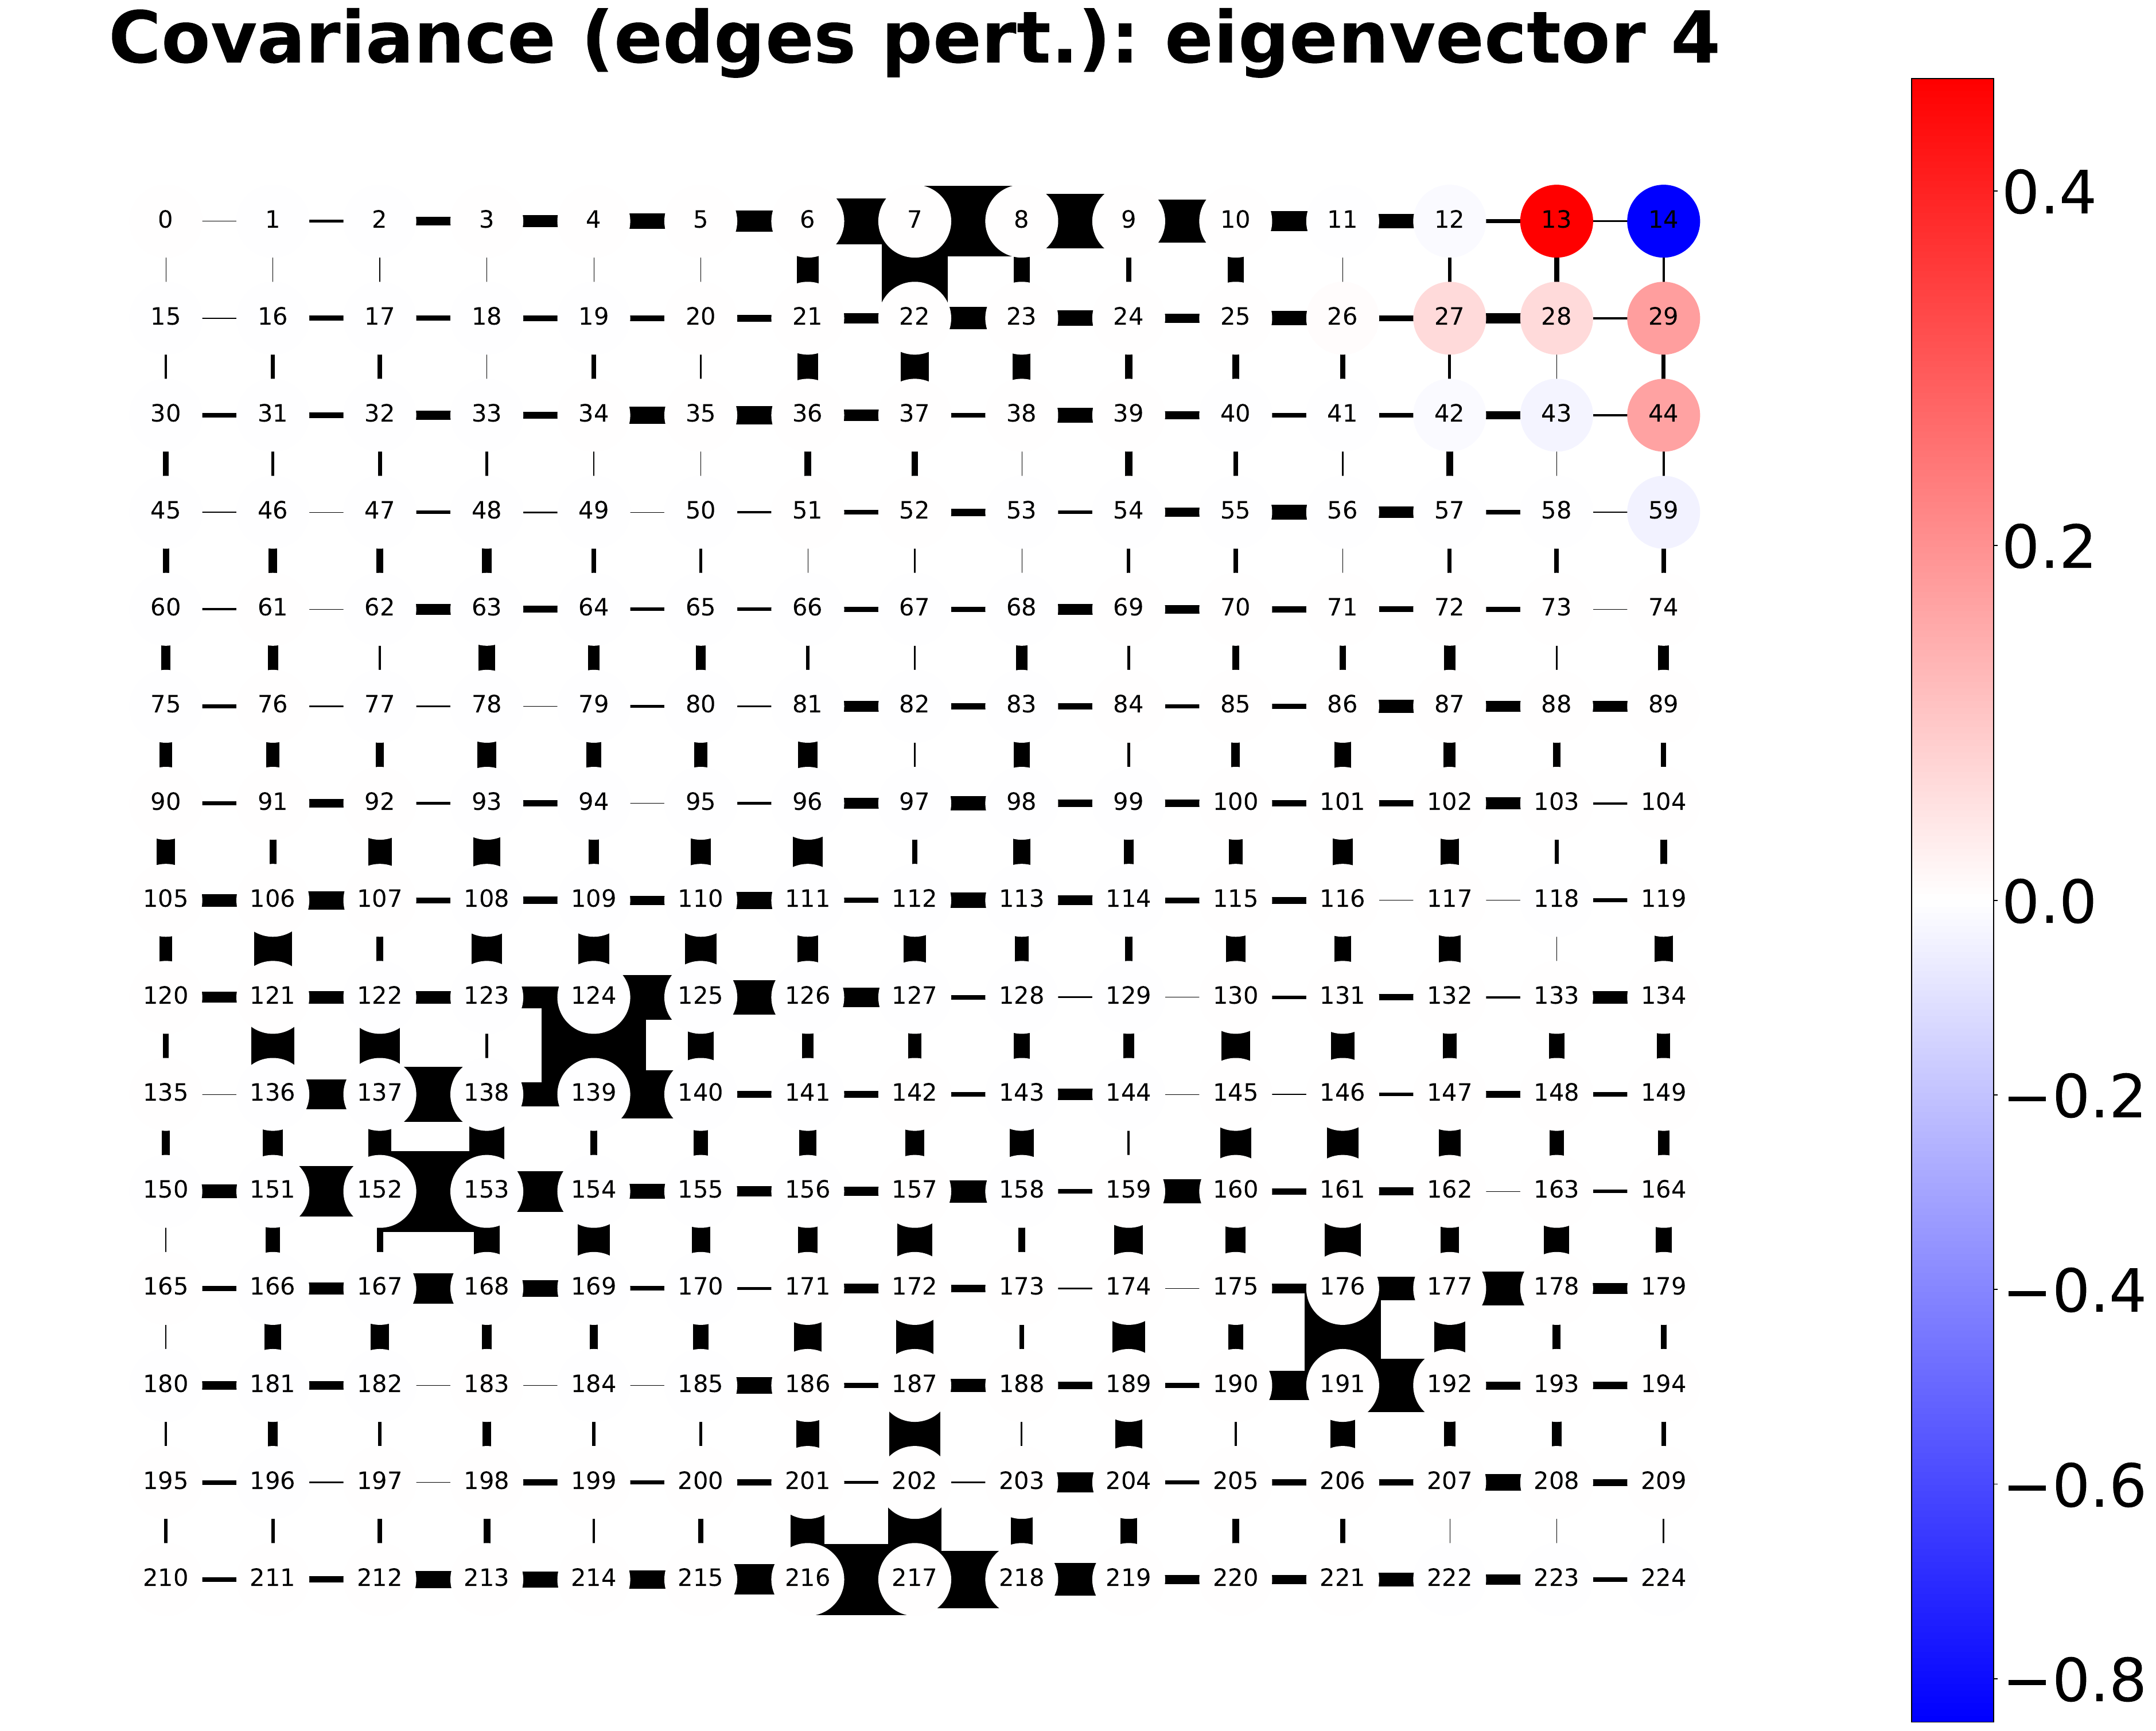}}
    \end{subfigure}

    \medskip
    
    \begin{subfigure}{.5\textwidth}
        {\centering
        \includegraphics[width=\linewidth]{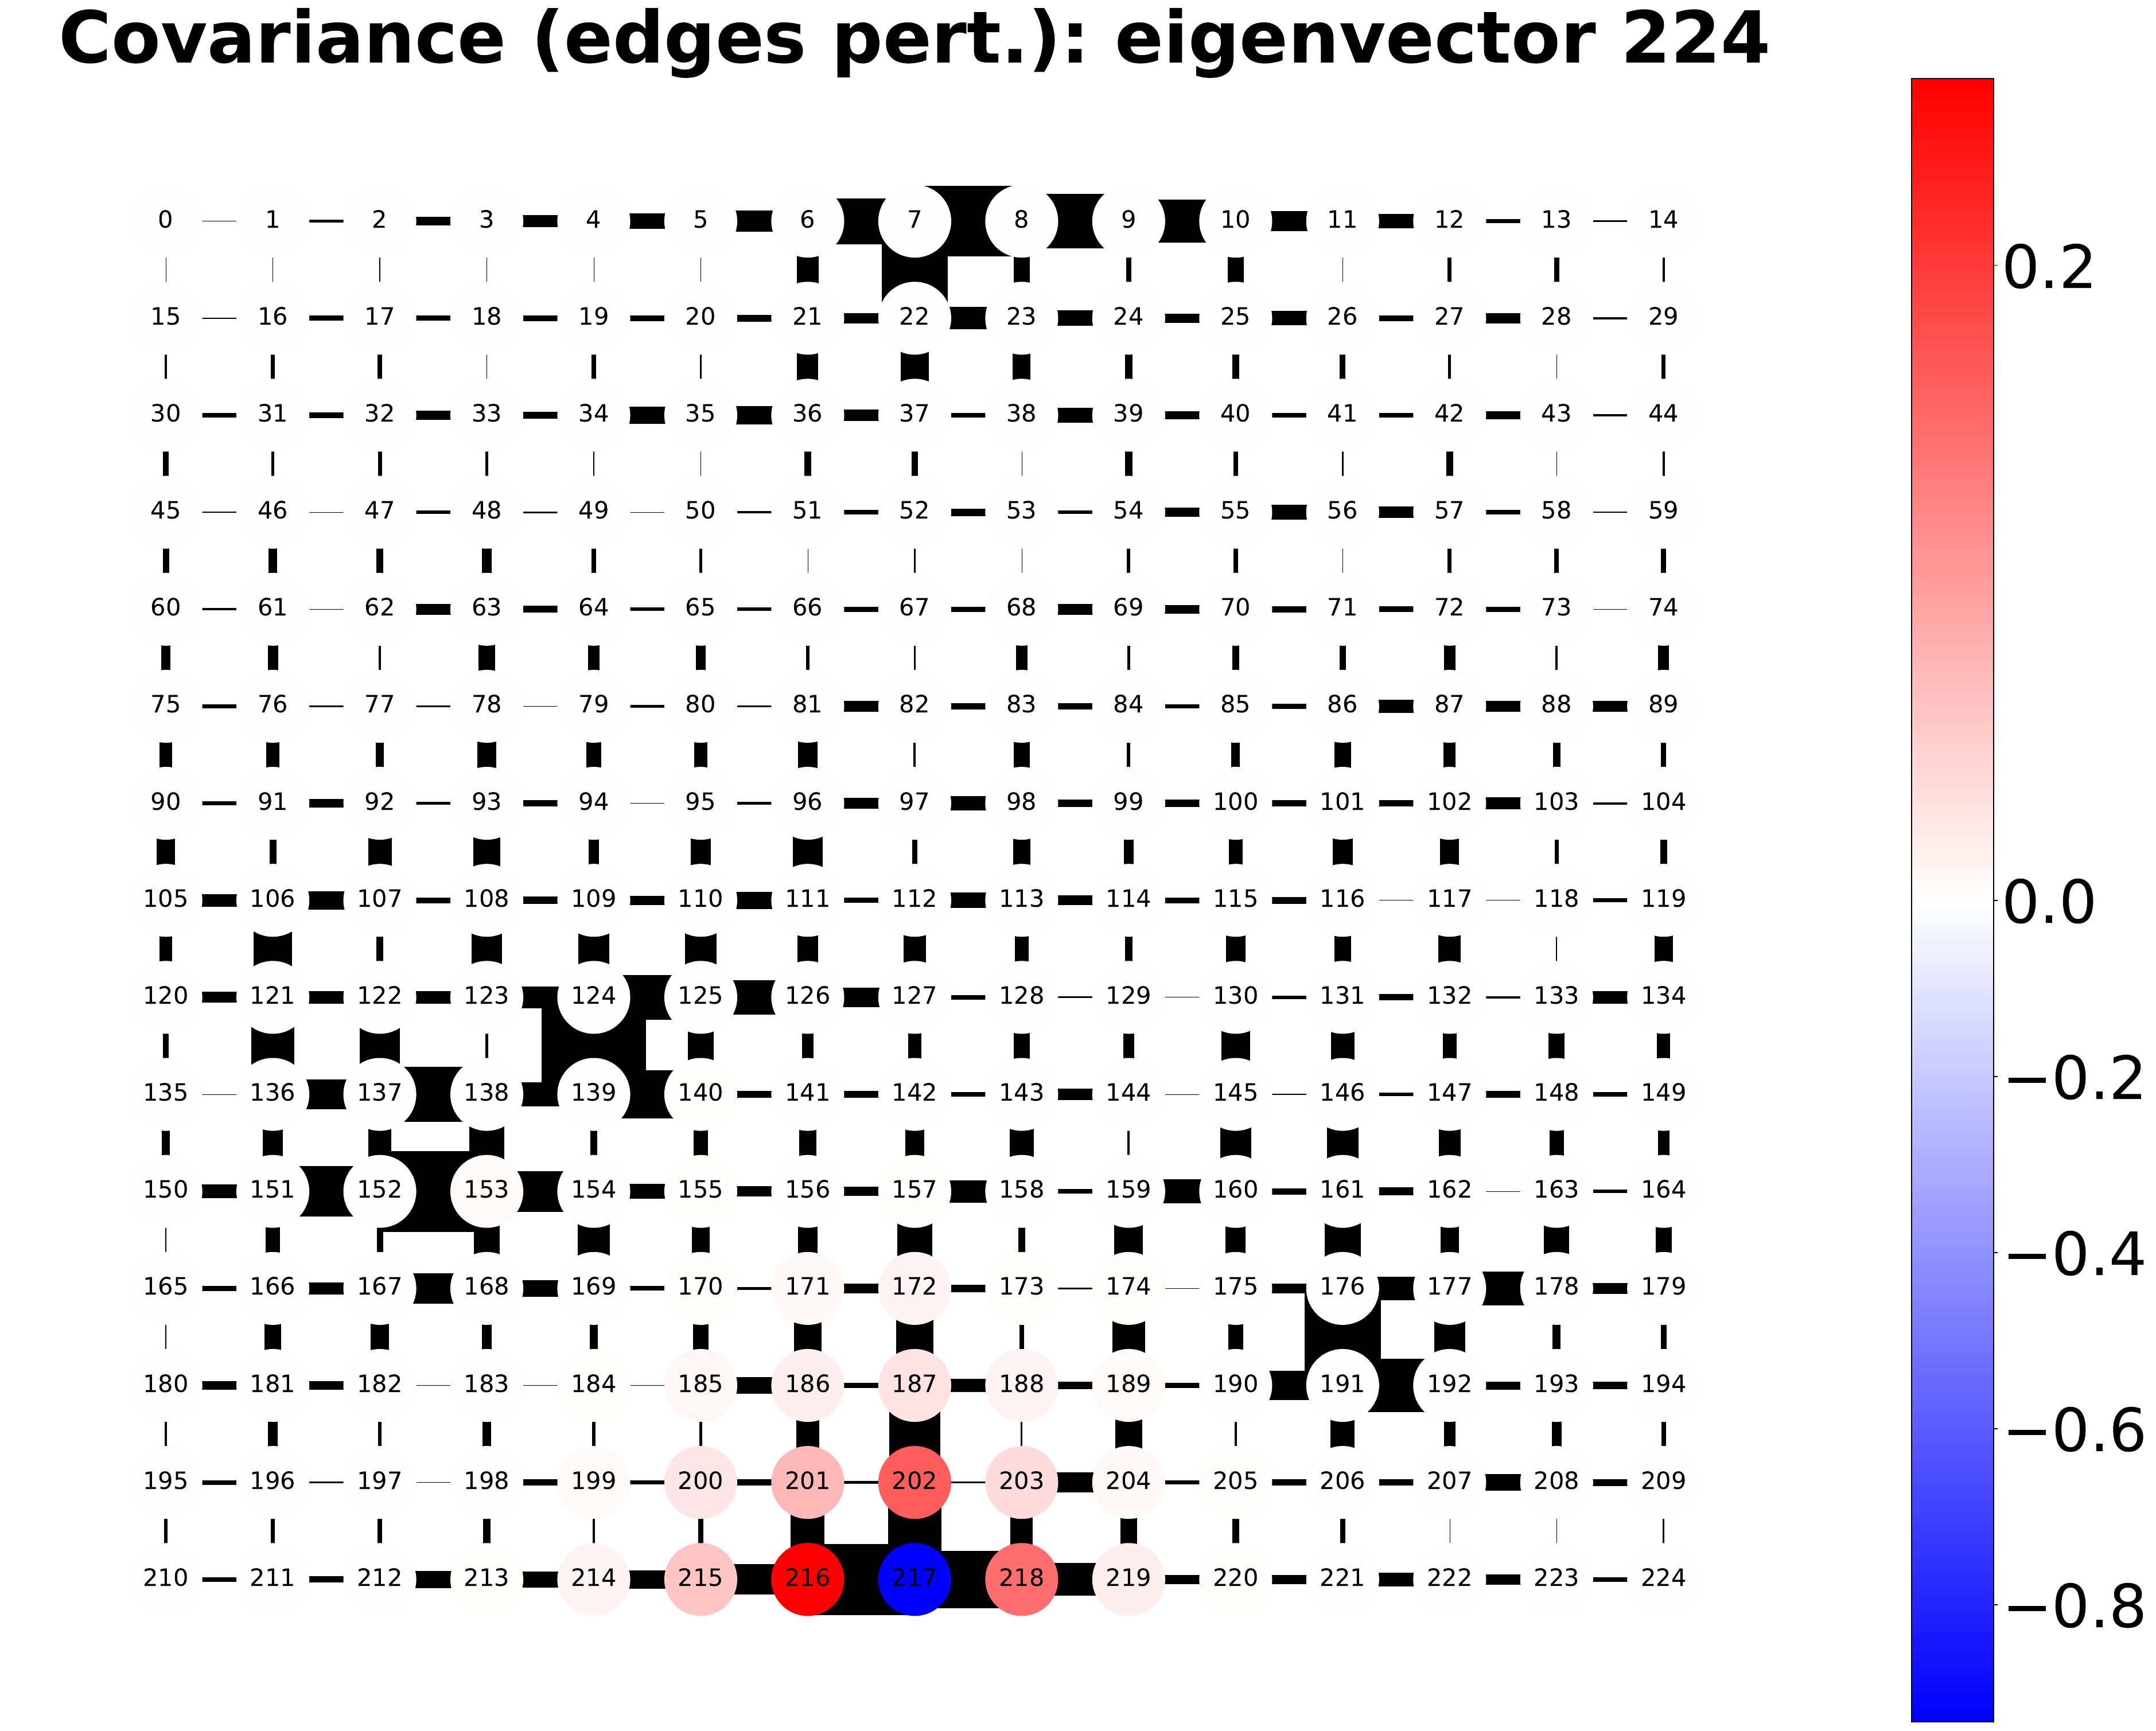}}
    \end{subfigure}\hfill % <-- "\hfill"
    \begin{subfigure}{.5\textwidth}
        {\centering
        \includegraphics[width=\linewidth]{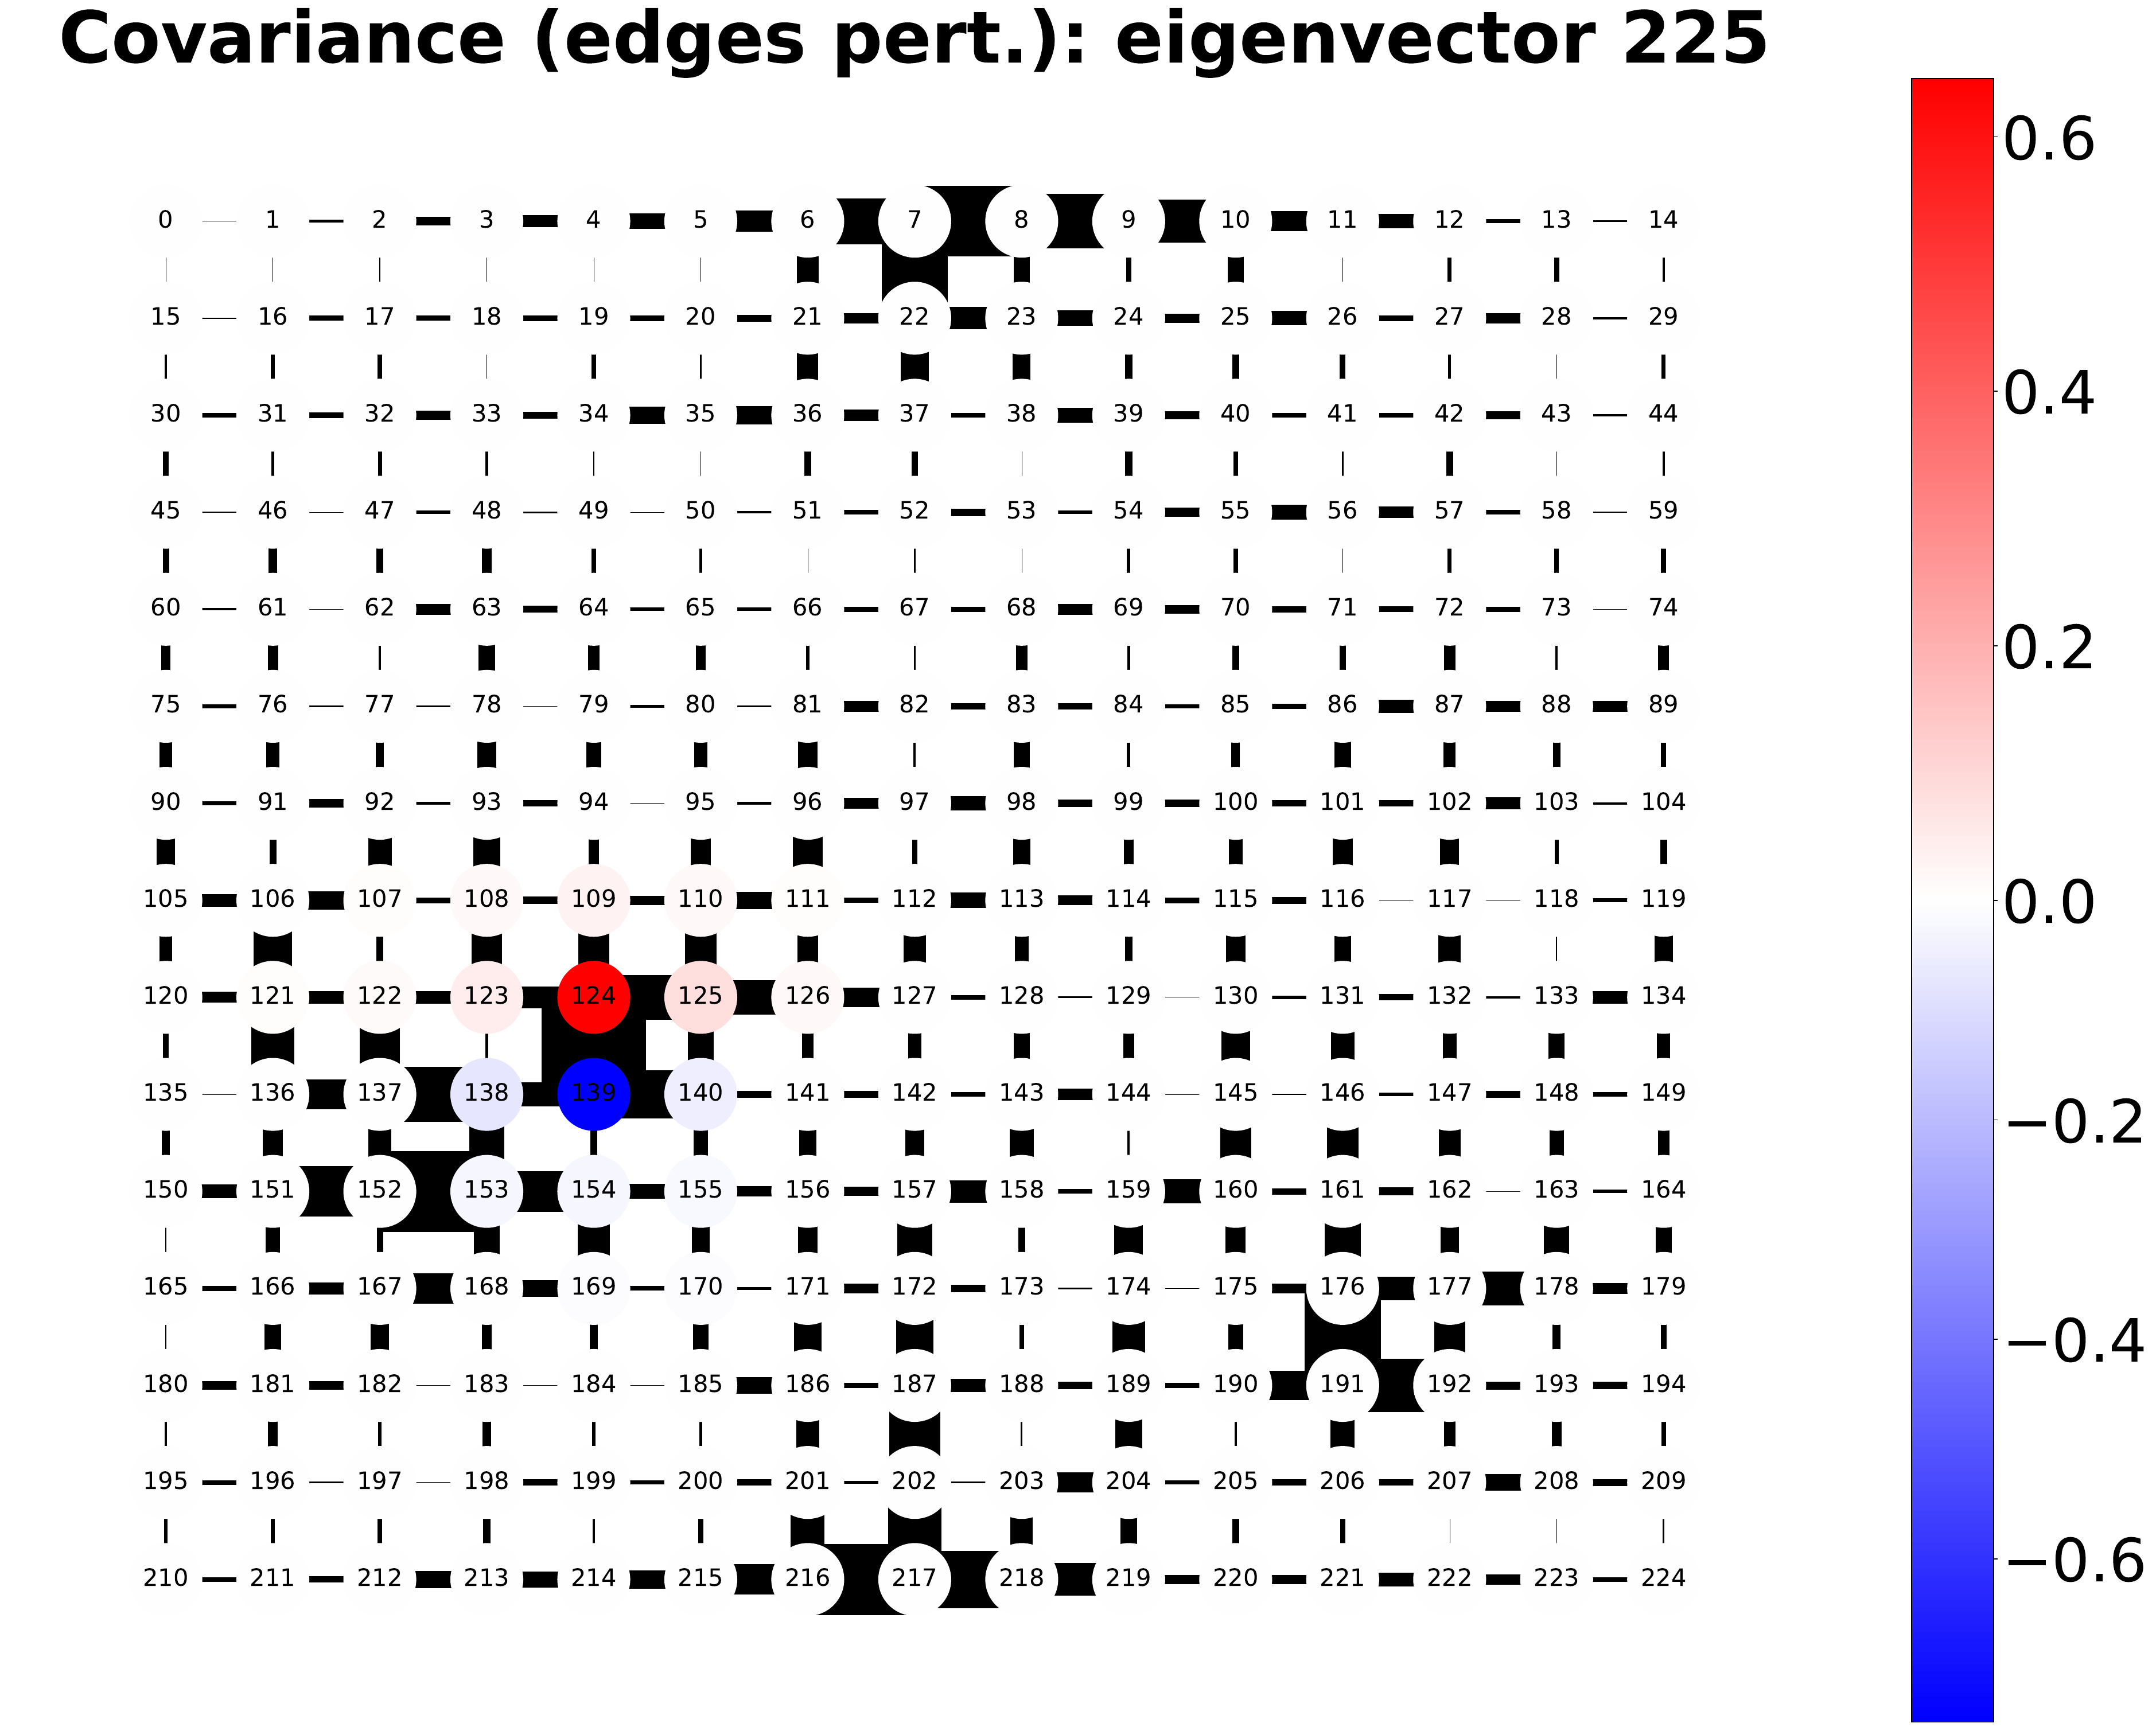}}
    \end{subfigure}
    \caption{In the figures we highlight the support nodes of the covariance matrix eigenvectors ordered according to the modulus of the eigenvalues. The relevance of the nodes is defined by the color scale on the right. The numbers give the stationary state of each nodes and the thickness of the links is proportional to the flux. We observe as the first eigenvectors are able to distinguish the links with lower fluxes (top pictures), whereas last eigenvectors distinguish links with higher fluxes (bottom pictures).}
    \label{fig:vector support}
\end{figure}

The covariance matrix associated to the transport network in presence of random link perturbations has the structure of a symmetric Laplacian matrix (i.e. each diagonal entry is the sum of the off diagonal elements so that its rows and columns sum to zero). This property follows by definition since the covariance matrix is computed on the eigenvectors of the Laplacian matrix of the network, that belong to the invariant subspace $\sum_k v_k=0$. Therefore the covariance matrix can be interpreted as the Laplacian matrix of an effective graph, derived from the initial one. The eigenvectors associated to the highest eigenvalues have support on the nodes connected by links with a great flux, whereas the ones associated to the lowest eigenvalues have support on the nodes connected by links with low flux. This property is illustrated by Fig. \ref{fig:vector support} for the grid network. The eigenvectors of the original Laplacian matrix have an analogous properties, but with respect to the link weight, and not to the link flux. Indeed, there is relation between the covariance among the node fluctuations and the weights of the connecting links. This is illustrated in Fig. \ref{fig:covariance matrix eigenvectors} for the grid network. This relation is at the basis of the traditional spectral clustering, that are less sensitive to the stationary fluxes among the links. Conversely, in the bottom part of the same figure we show as the proposed approach which considers the node covariance properties due to the fluctuations in the link weights, is related to the flux magnitude along the links, whereas is less sensitive to the link weights. In this way we realize a different spectral clustering. Similar results hold for the different graph topology considered in the paper.

% Correlation vs edge weight/fluc and Variance vs node strength/netflux
\begin{figure*}[!htb]
    \centering
    \includegraphics[width=0.9\textwidth]{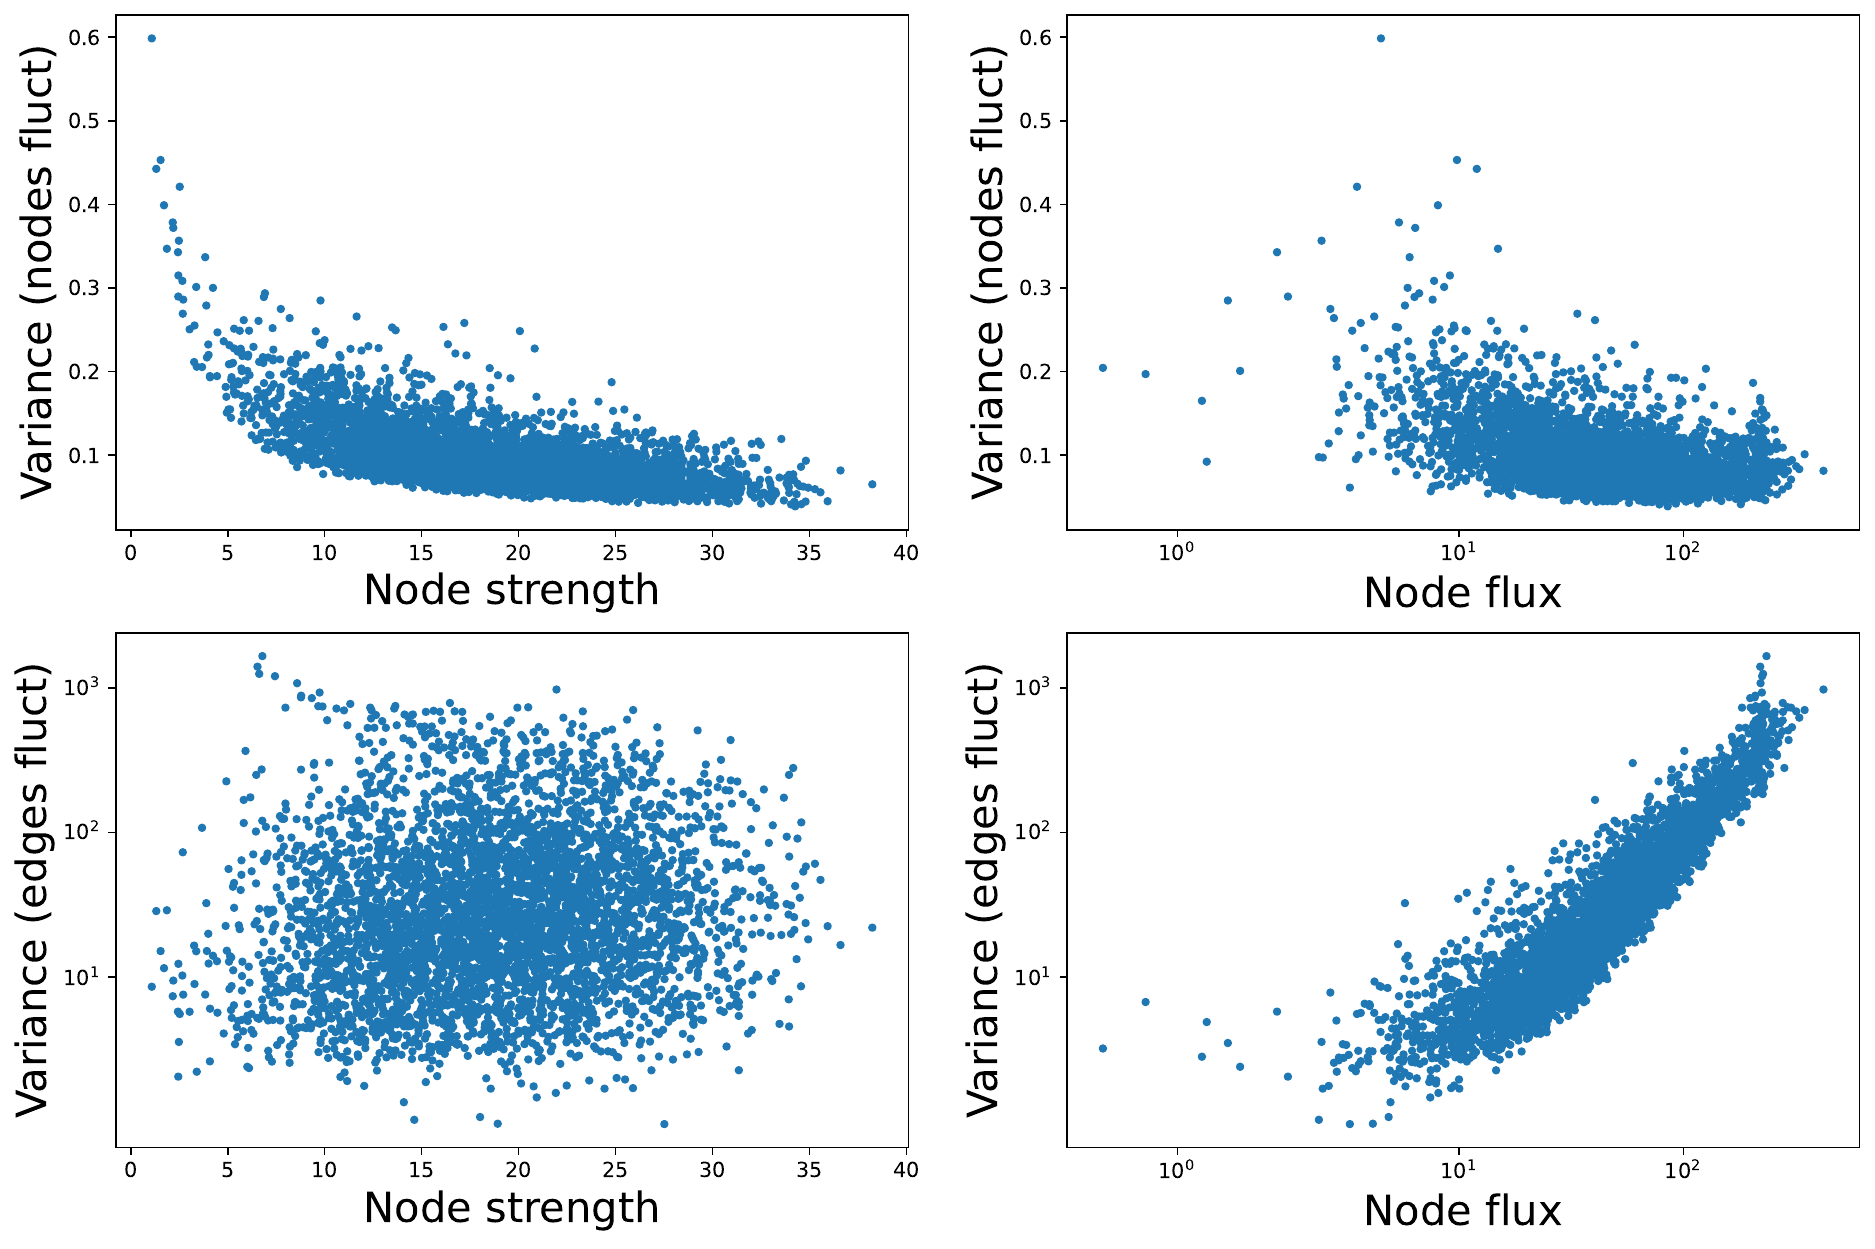}
    \caption{The top-left picture highlights the relation between the fluctuations of the node state in a grid network and the edge weights that is exploited in the traditional spectral clustering, whereas the top-right picture shows that these fluctuations are less sensitive to the stationary link fluxes.  On the contrary, the covariance among the node states due to the link fluctuations are poorly related with the link weight (the bottom-left picture) and greatly related to the link fluxes (bottom-right picture).  (This property is exploited by the proposed PC embedding + k-medoid clustering method).}
    \label{fig:covariance matrix eigenvectors}
    
\end{figure*}
 
%\begin{figure*}[!htb]
%    \centering
%    \includegraphics[width=0.9\textwidth]{pictures/Variance_Grid.pdf}
%    \caption{Grid network. There is a correlation between the variance in the edges perturbation covariance matrix and the nodes flux (sum of the incoming and outgoing fluxes).}
    %\label{fig:grid-all edges}
%\end{figure*}
%%%%%%%%%%%%%%%%%%%%%%%%%%%%%%%%%%%%%%%%%%%%%%%%%%%%%%%%%

The clustering procedure proposed in the main text put together the nodes with positive covariance among them. Moreover, the nodes with with negative correlation values among them (corresponding generally to higher fluxes, as seen above) are attributed to different clusters. A structure-based clustering method, like the Louvain method, applied on the same transport network, does not distinguish between positive and negative correlation, since the information on the correlation is not present, and, more importantly, it has no information about the fluxes of the network, which we are interested in. In Fig. \ref{fig:heatmap_regular} and Fig. \ref{fig:heatmap_grid}  we illustrate the clustering procedure using an heatmap for a realization of a 4-regular network and a grid, comparing the clustering results using the Louvain method. The obtained clusters are highlighted by black squares on the main diagonal.   
\clearpage
\begin{figure}[h]
    \centering
    \includegraphics[width=0.5\textwidth]{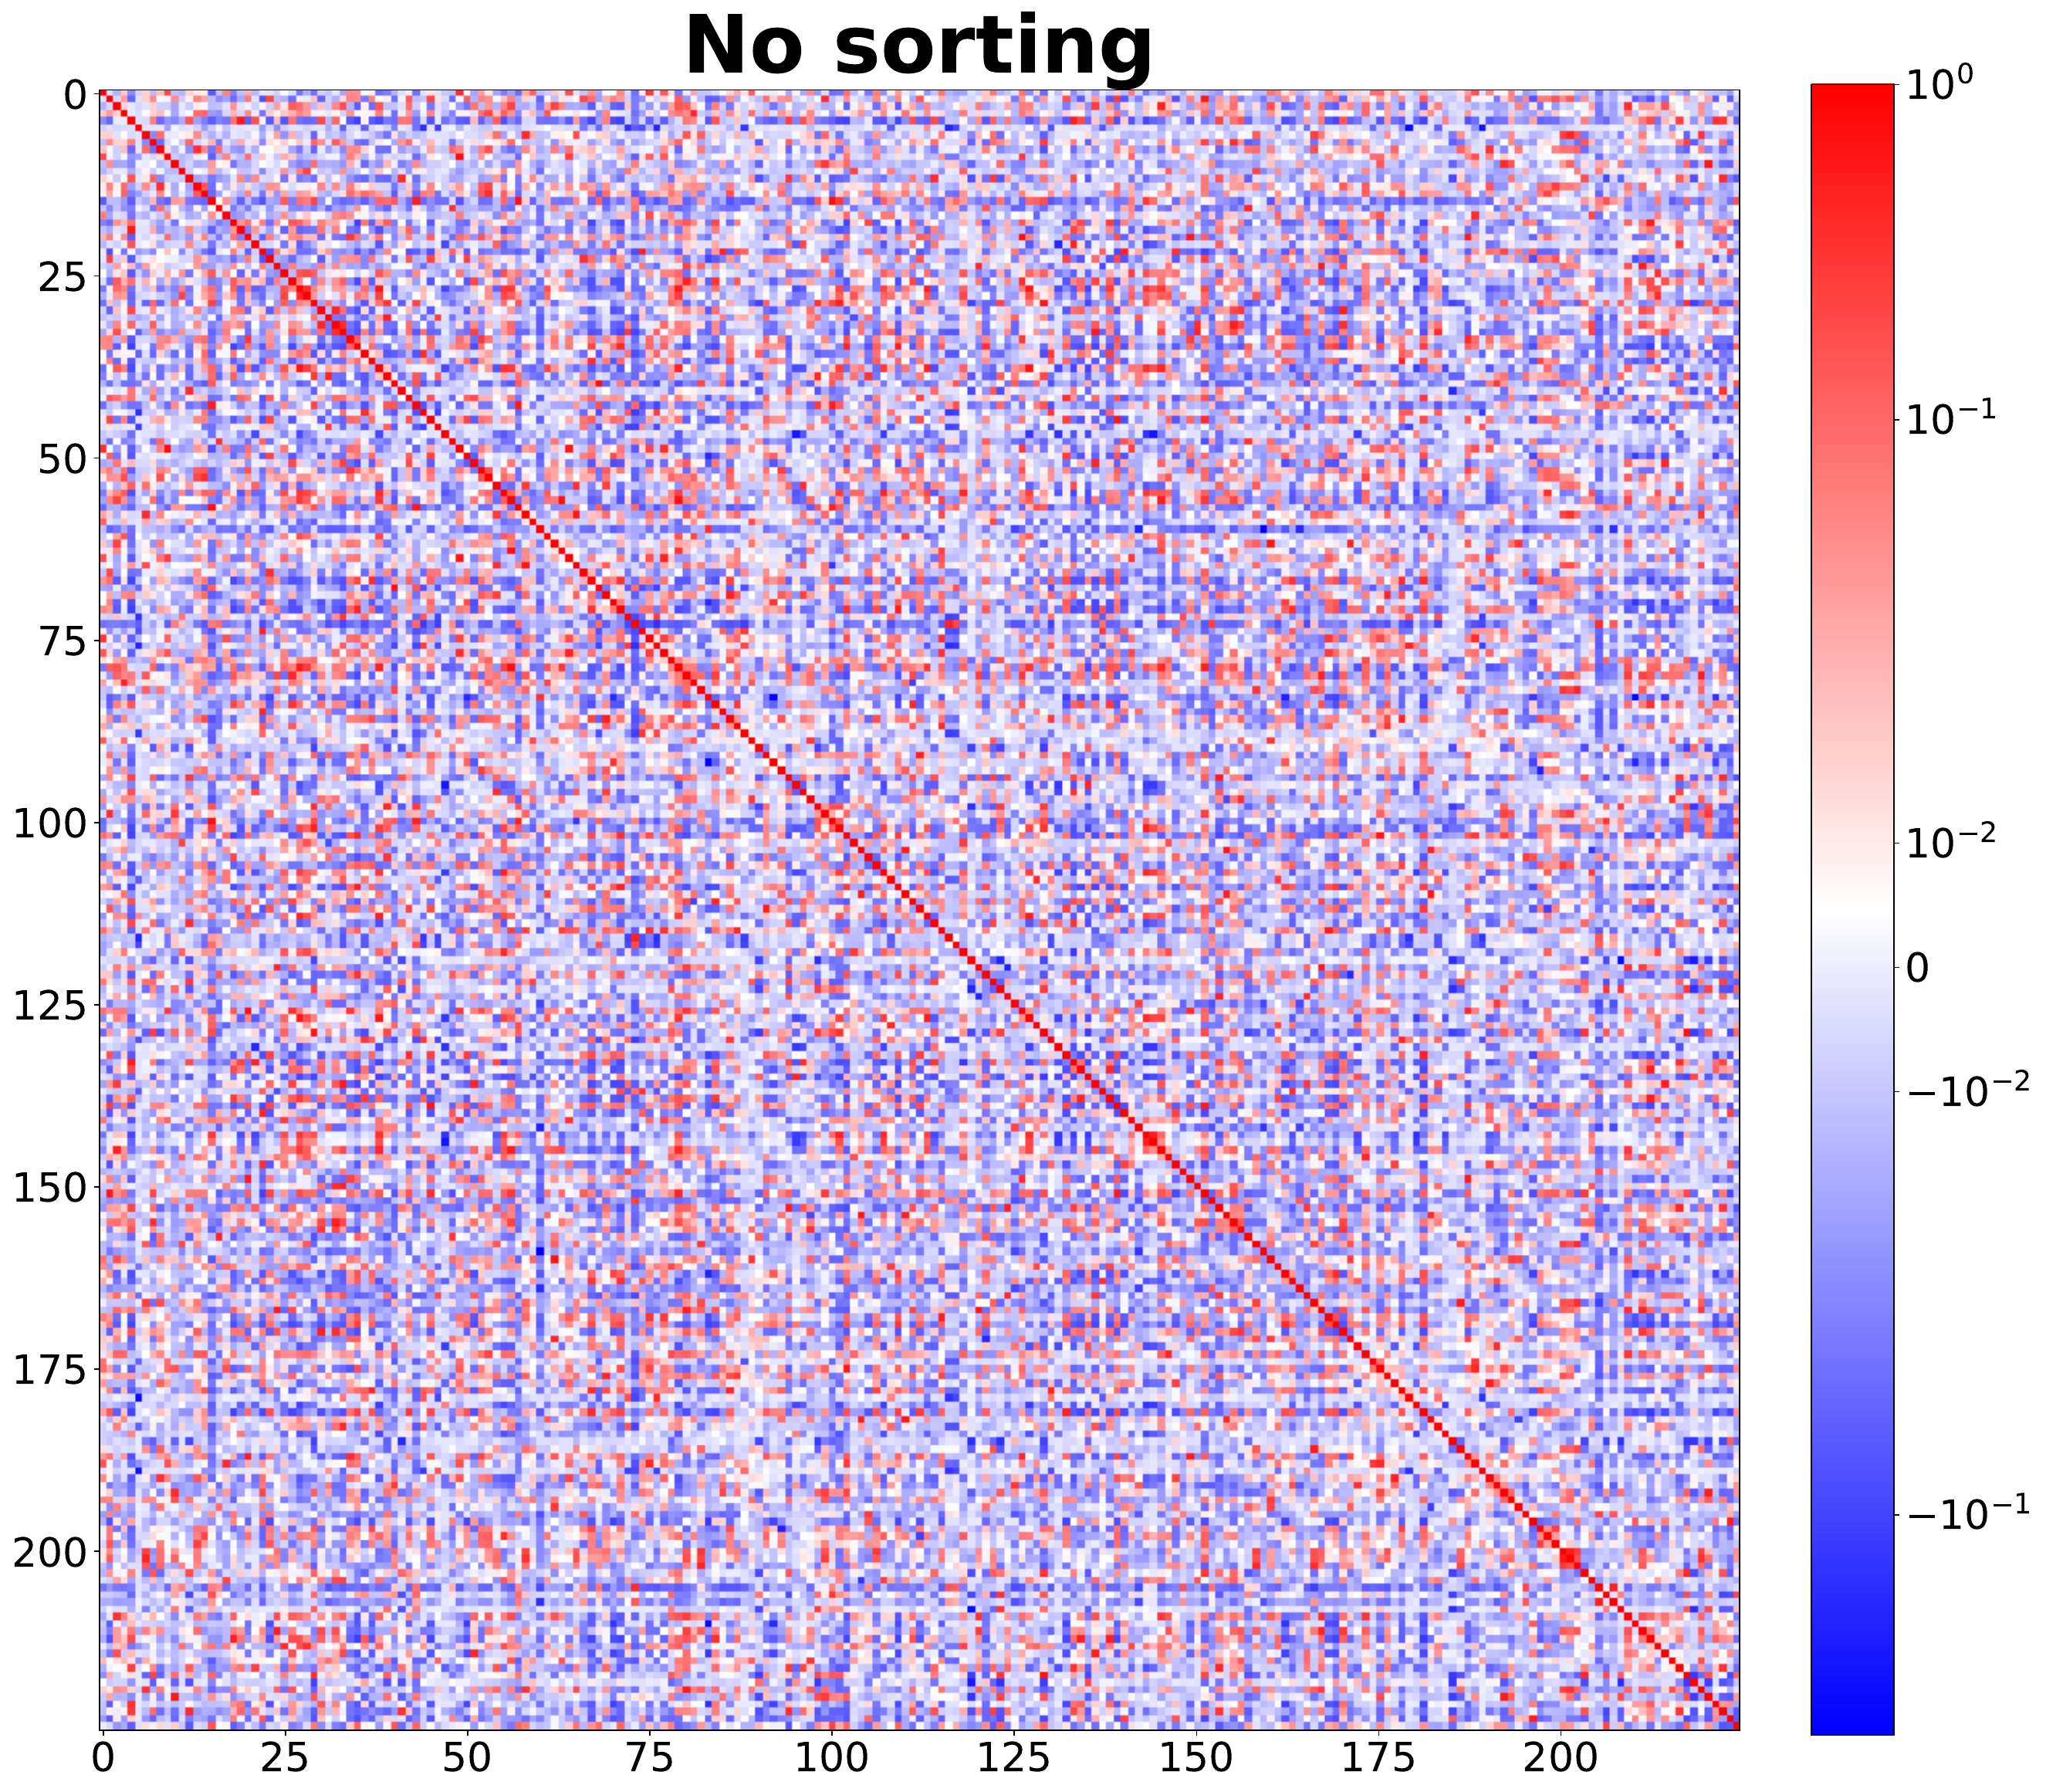}
\end{figure}

\begin{figure}[h]
    \centering
    \includegraphics[width=1\textwidth]{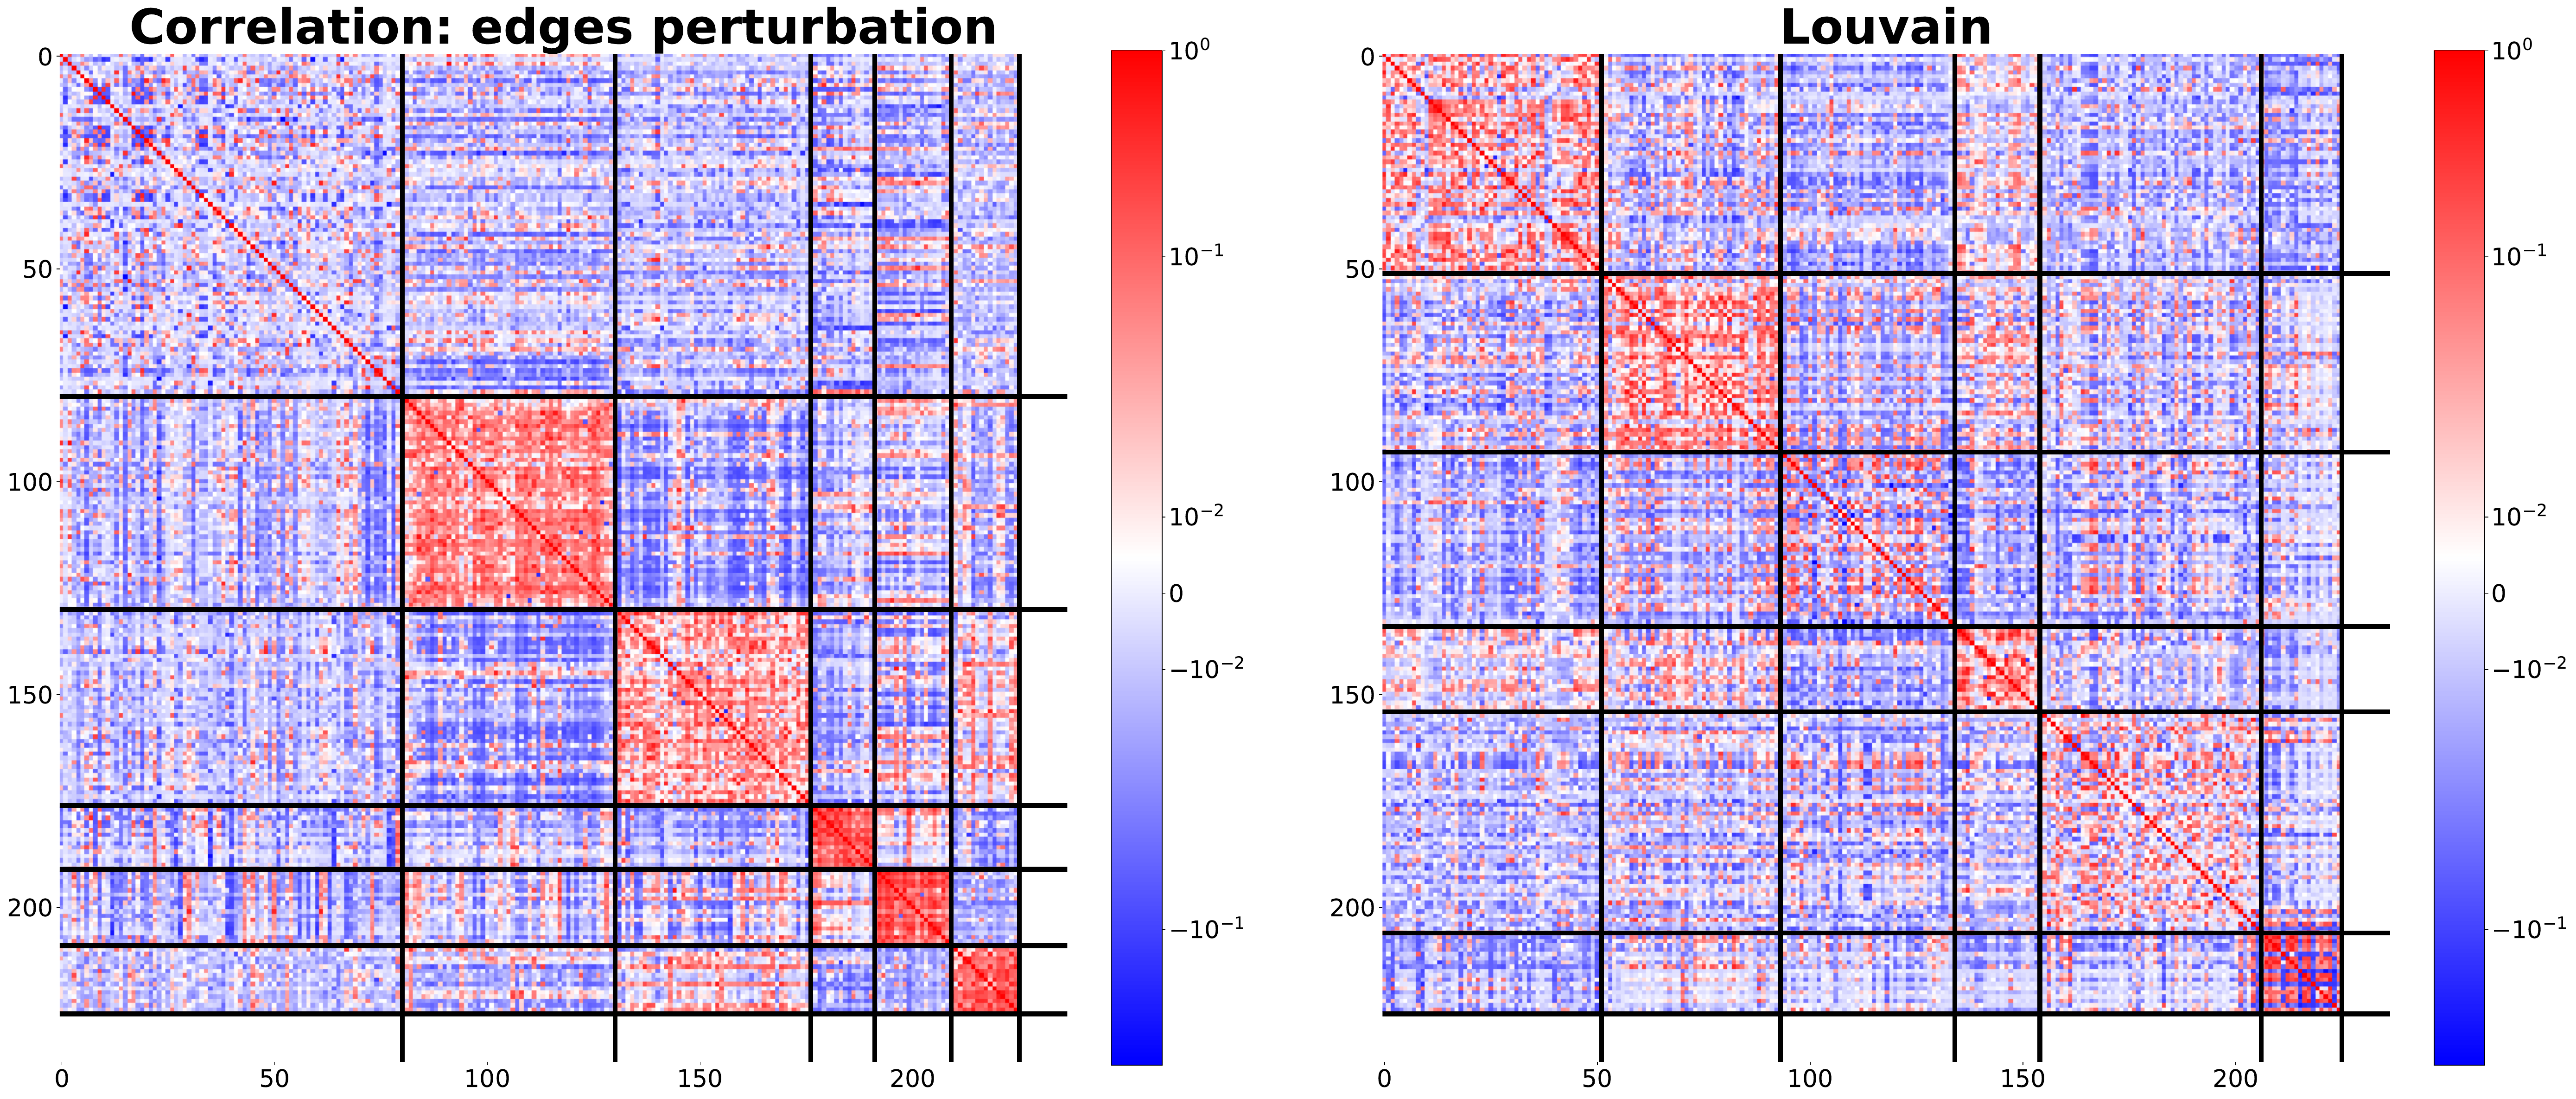}
    \caption{Clustering for a realization of a 4-regular transport network. The first heatmap (top picture) is the covariance matrix computed by eq. (21) in the main text. The covariance value is encoded by the color scale shown on the right. The bottom heatmaps are the result of a sorting procedure according to the clusters created by the proposed method (left picture) and the Louvain method (right picture). Each cluster corresponds to a diagonal square with black borders. The off-diagonal rectangles correspond to the negative correlation values among nodes belonging to different clusters.}
\label{fig:heatmap_regular}    
\end{figure}
\clearpage
\begin{figure}[h]
    \centering
    \includegraphics[width=0.5\textwidth]{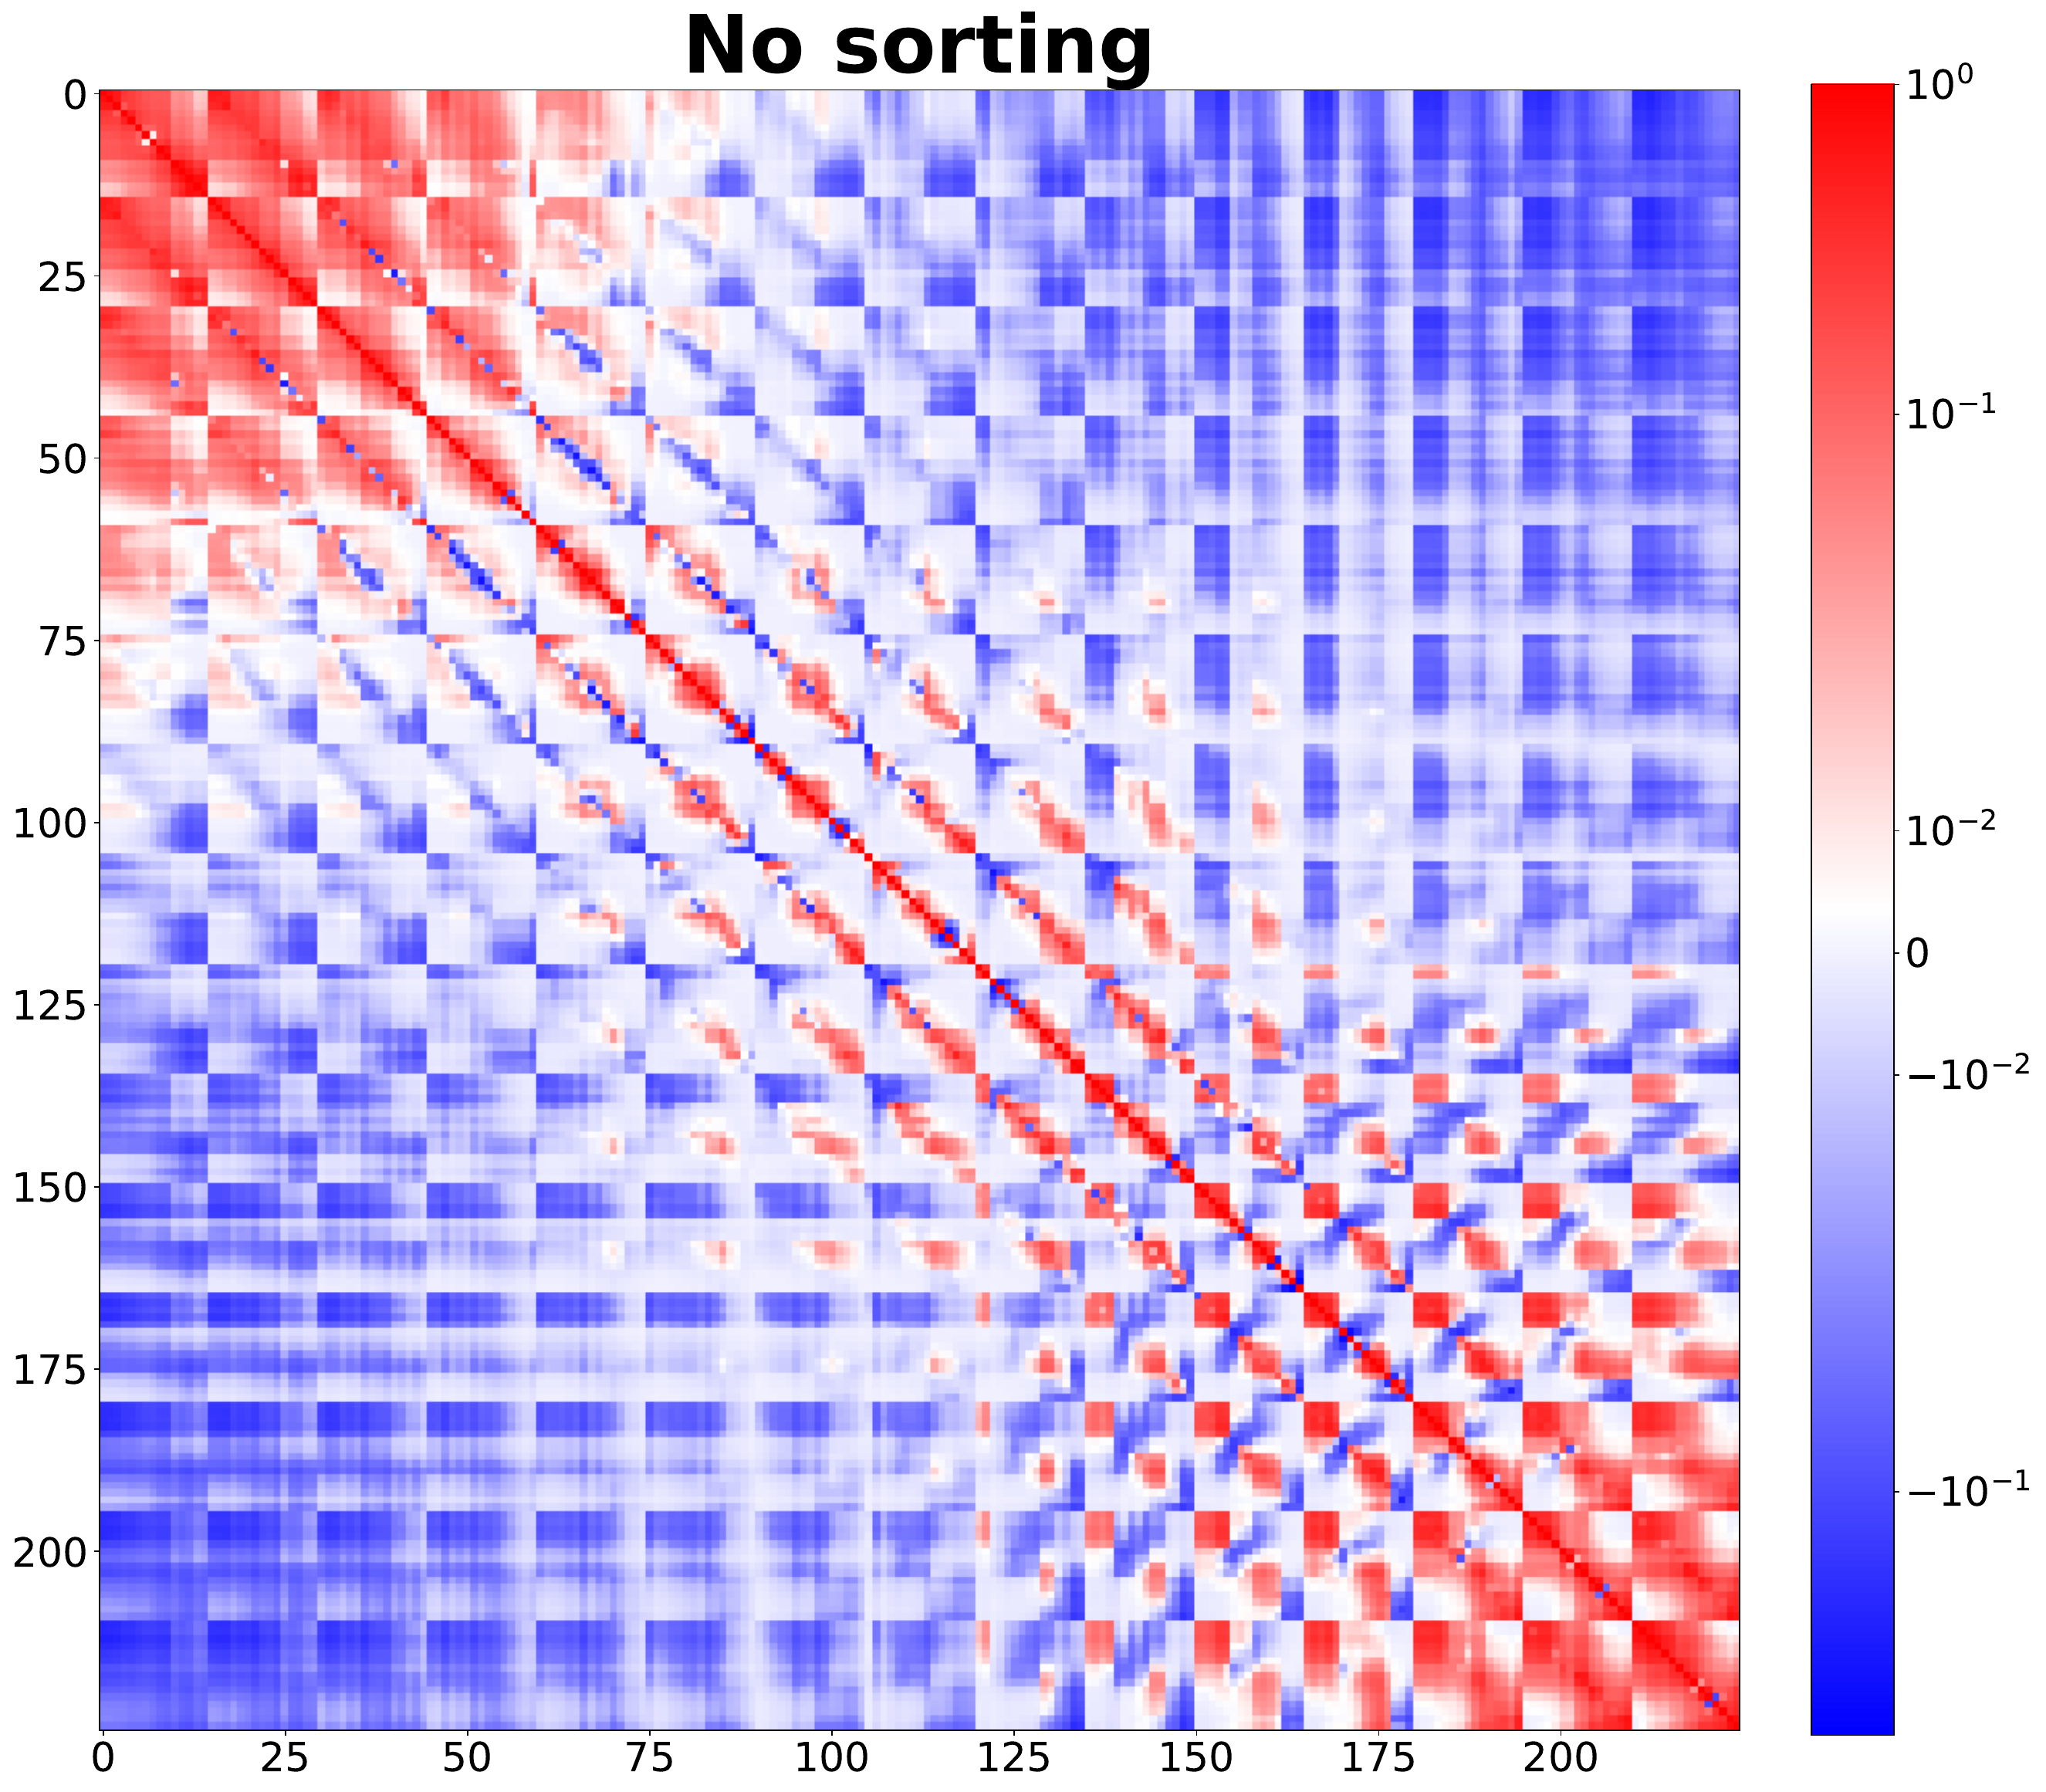}
\end{figure}
\begin{figure}[h]
    \centering
    \includegraphics[width=1\textwidth]{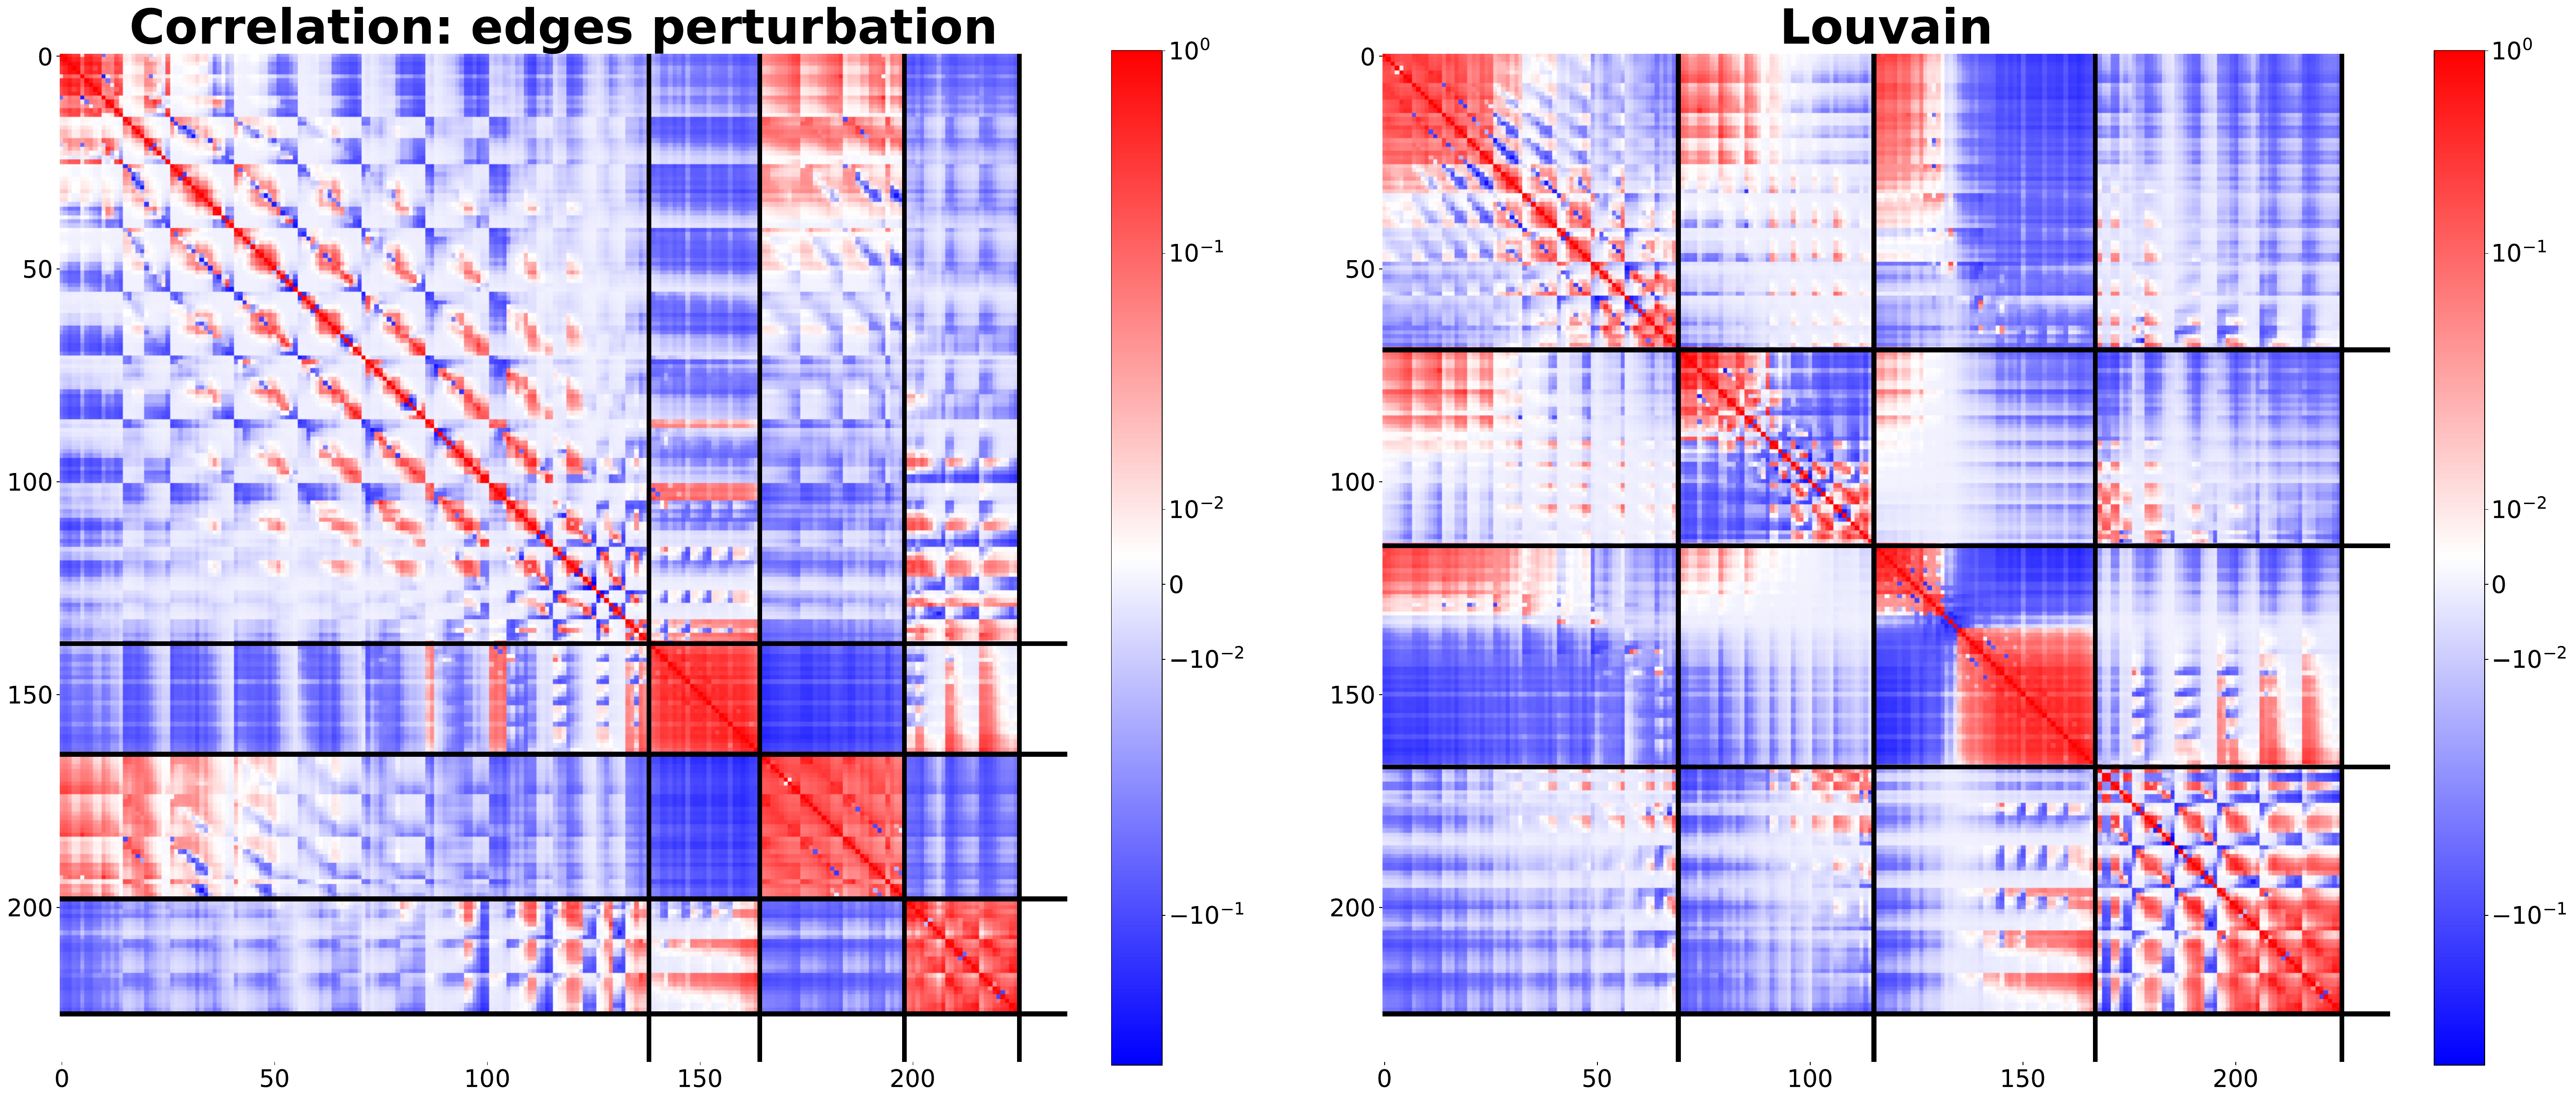}
    \caption{Clustering for a realization of Grid network. The explanation of the heatmaps is the same as in Fig. \ref{fig:heatmap_regular}.}
\label{fig:heatmap_grid}    
\end{figure}

We have validated the efficiency of proposed approach to detect the link failures in transport network by computing the efficiency value (cfr. eq. (31) in the main text) averaged over 20 realisations of different network topologies. We have considered the correlation and covariance matrices of the network under different types of perturbations and we have compared oue results with the modularity maximization clustering method (Louvain
method) and the algorithm by Girvan and Newman, to detects the communities (see the main text). To complete the discussion of the section VII in the main text, we report in the Fig. \ref{fig:barabasi-edges} and 6 the results for the Barabasi-Albert scale free random network and the 4-regular network, analogous to those shown in the figure 5 of the main text. We compare the efficiency of the failure detection methods when the failure may occur in any link and when we restrict this possibility to the link with higher flows. In the last case the propose method based on the covariance matrix when the links are randomly perturbed turns out to be more efficient for all the considered network topologies.
\begin{figure*}[!htb]
    \centering{
    \includegraphics[width=0.8\textwidth]{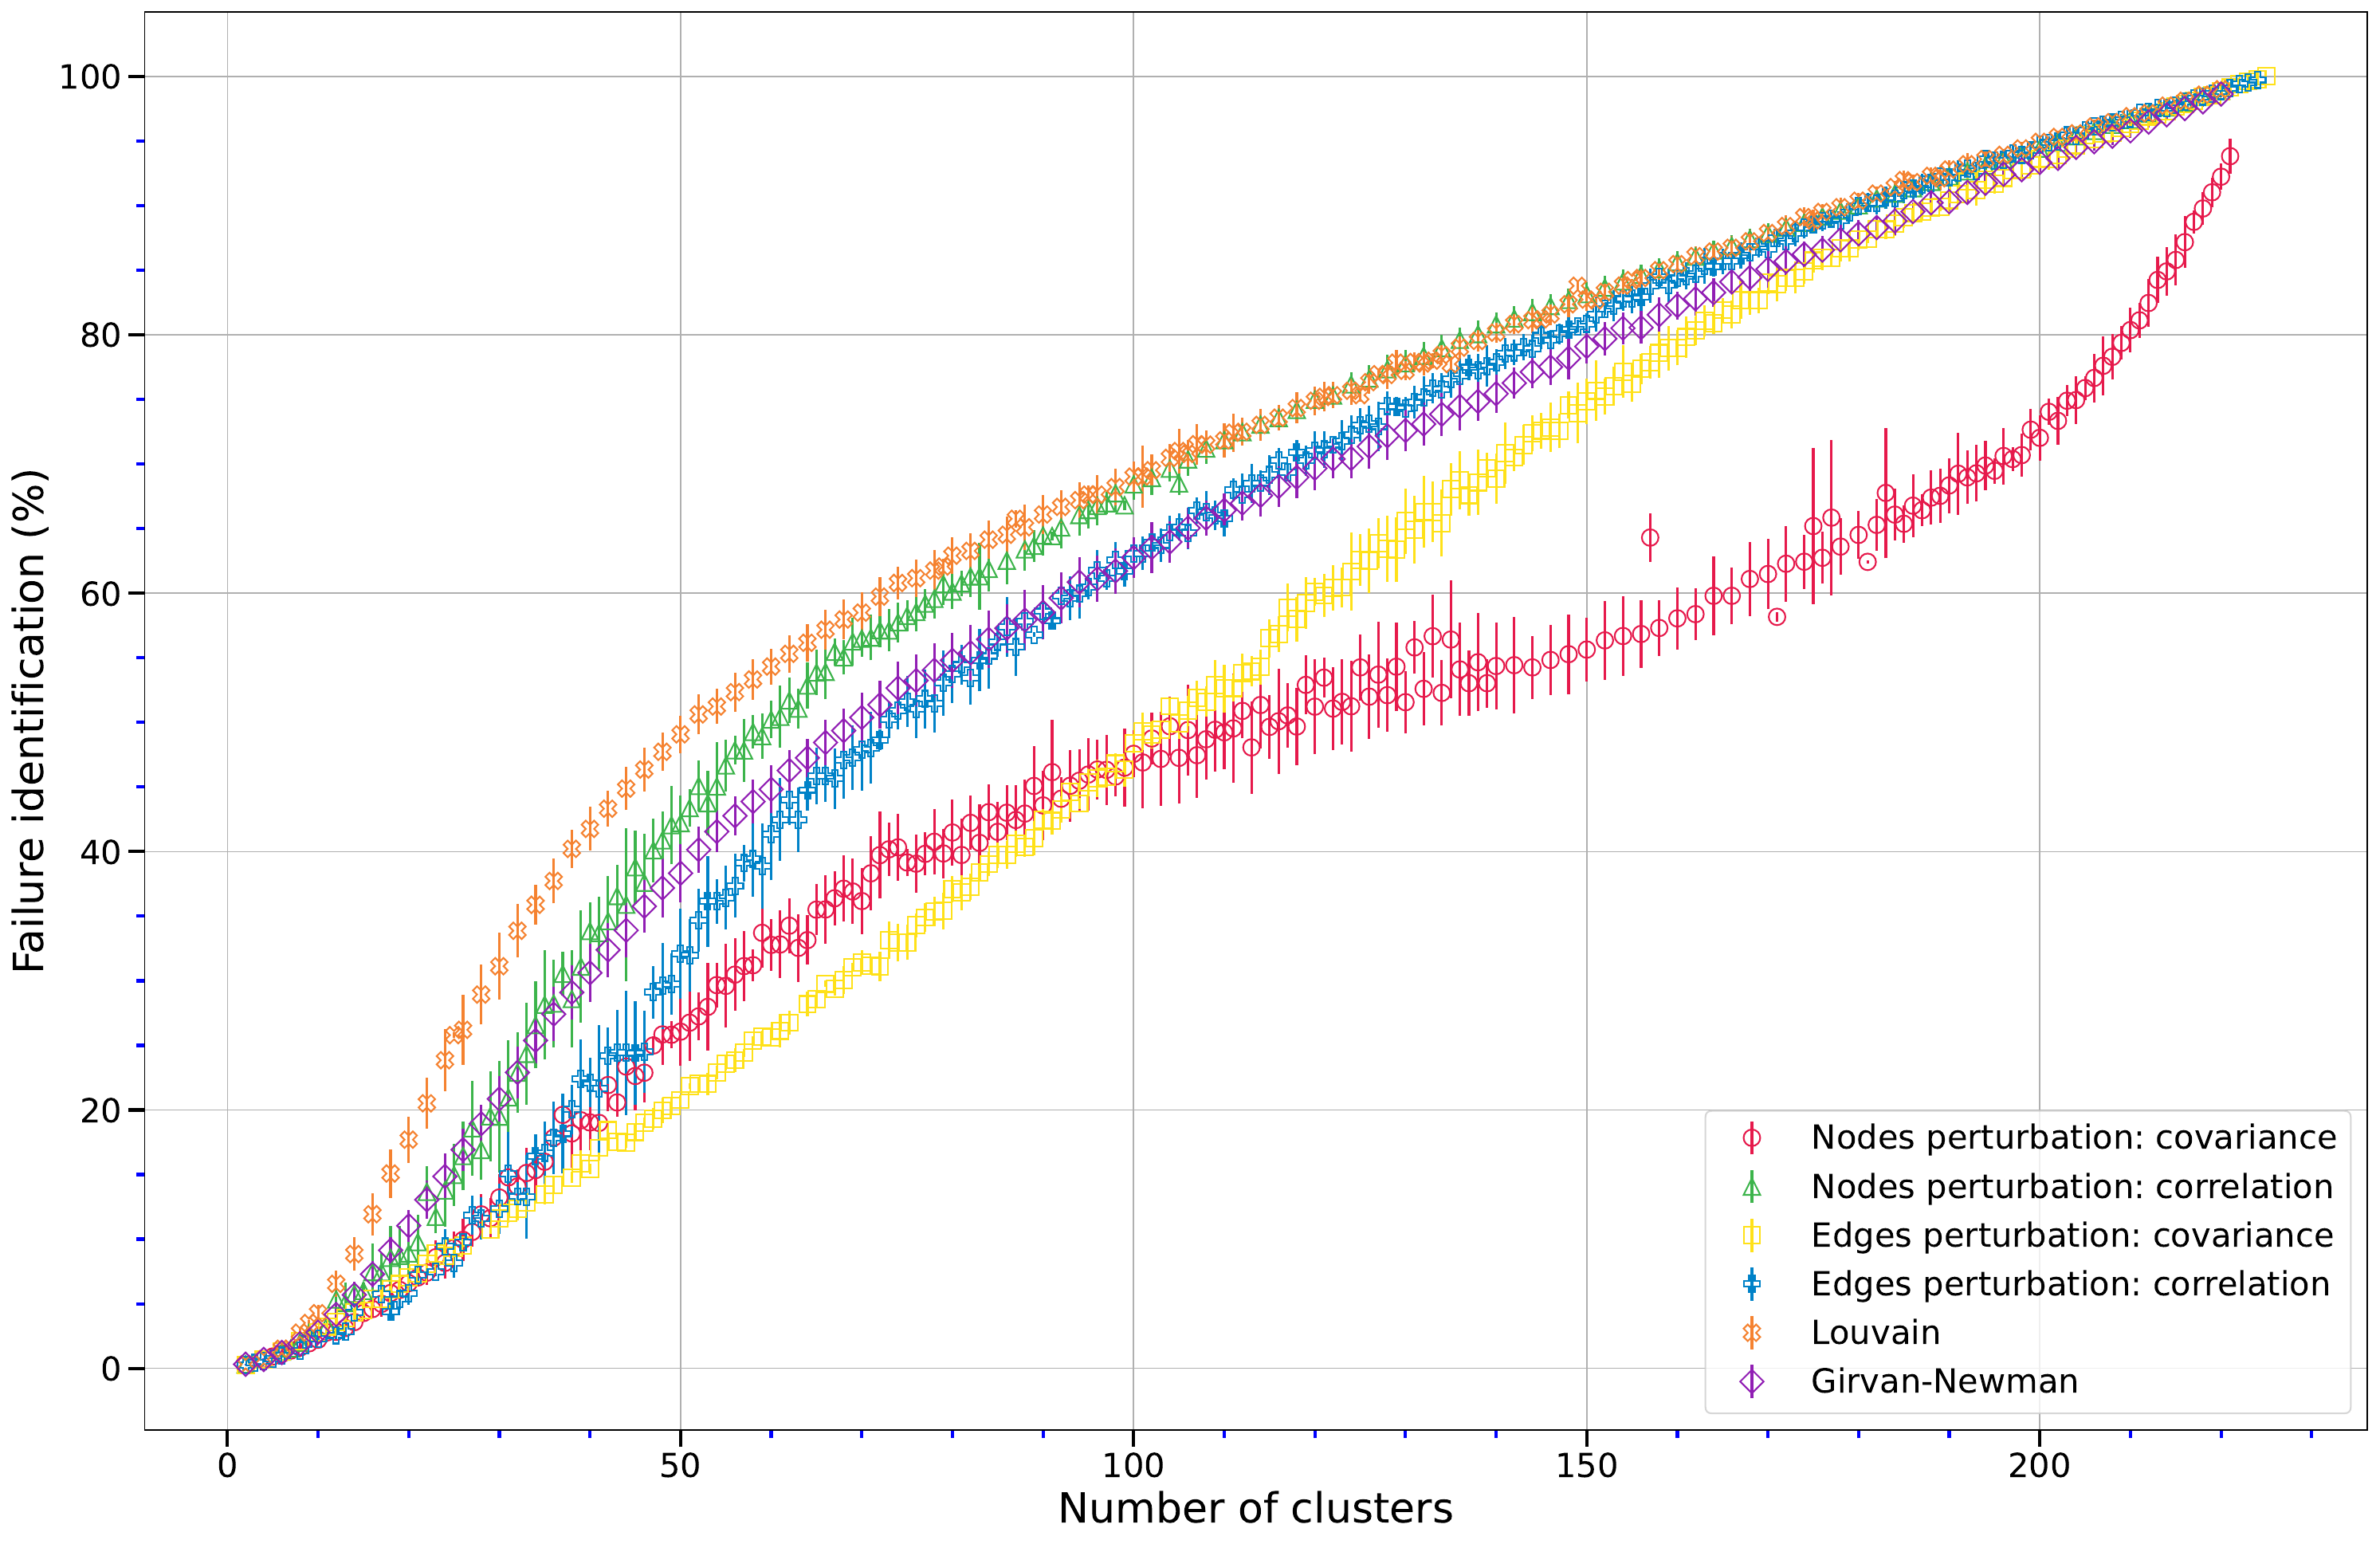}}
\end{figure*}
\begin{figure*}[!htb]
    {\centering
    \includegraphics[width=0.8\textwidth]{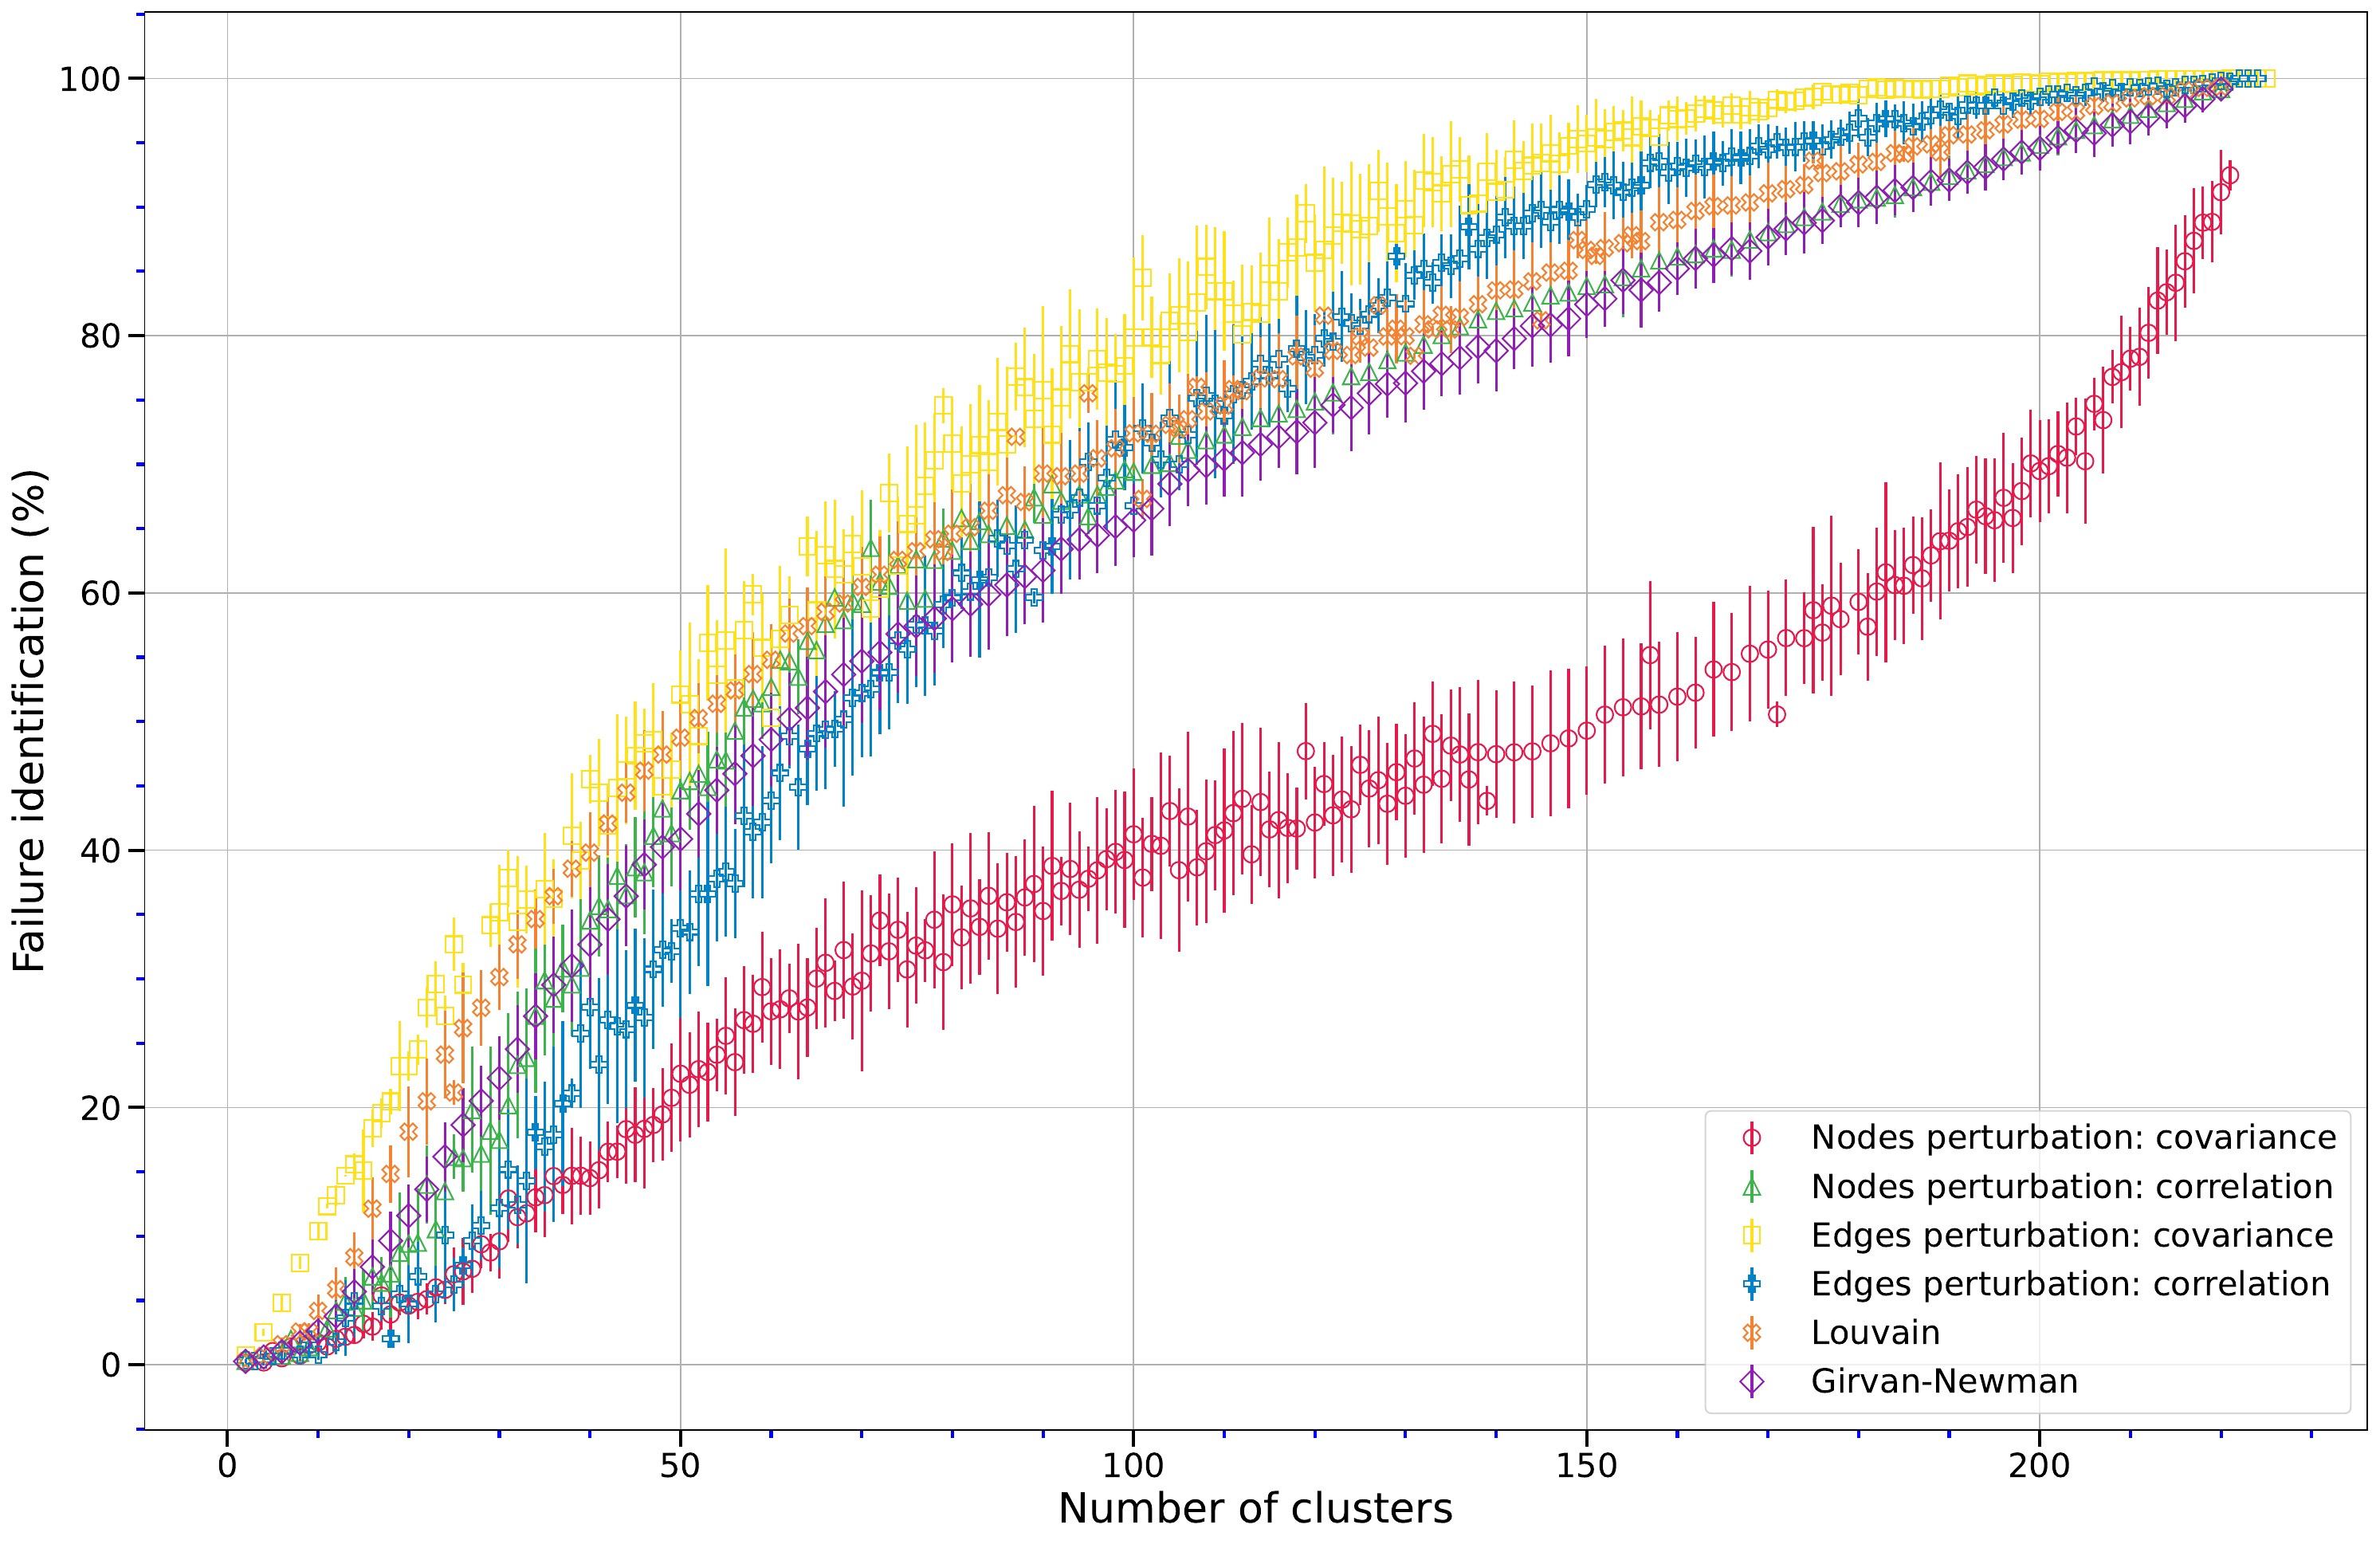}}
\caption{Failure detection efficiency (cfr. eq. (35) in the main text) as a function of clusters number for the Barabasi-Albert random network with $225$ nodes and average degree $k=4$. The results are averaged over 20 realizations
of the network structure reporting the standard deviation on each point. In the top figure we show detection efficiency over
all the possible single-edge failures. In the bottom figure we show detection efficiency over the edges, whose flow value is more
than the 75-th percentile of the flow distribution. }
\label{fig:barabasi-edges}
\end{figure*}

\begin{figure*}[!htb]
    {\centering
    \includegraphics[width=0.8\textwidth]{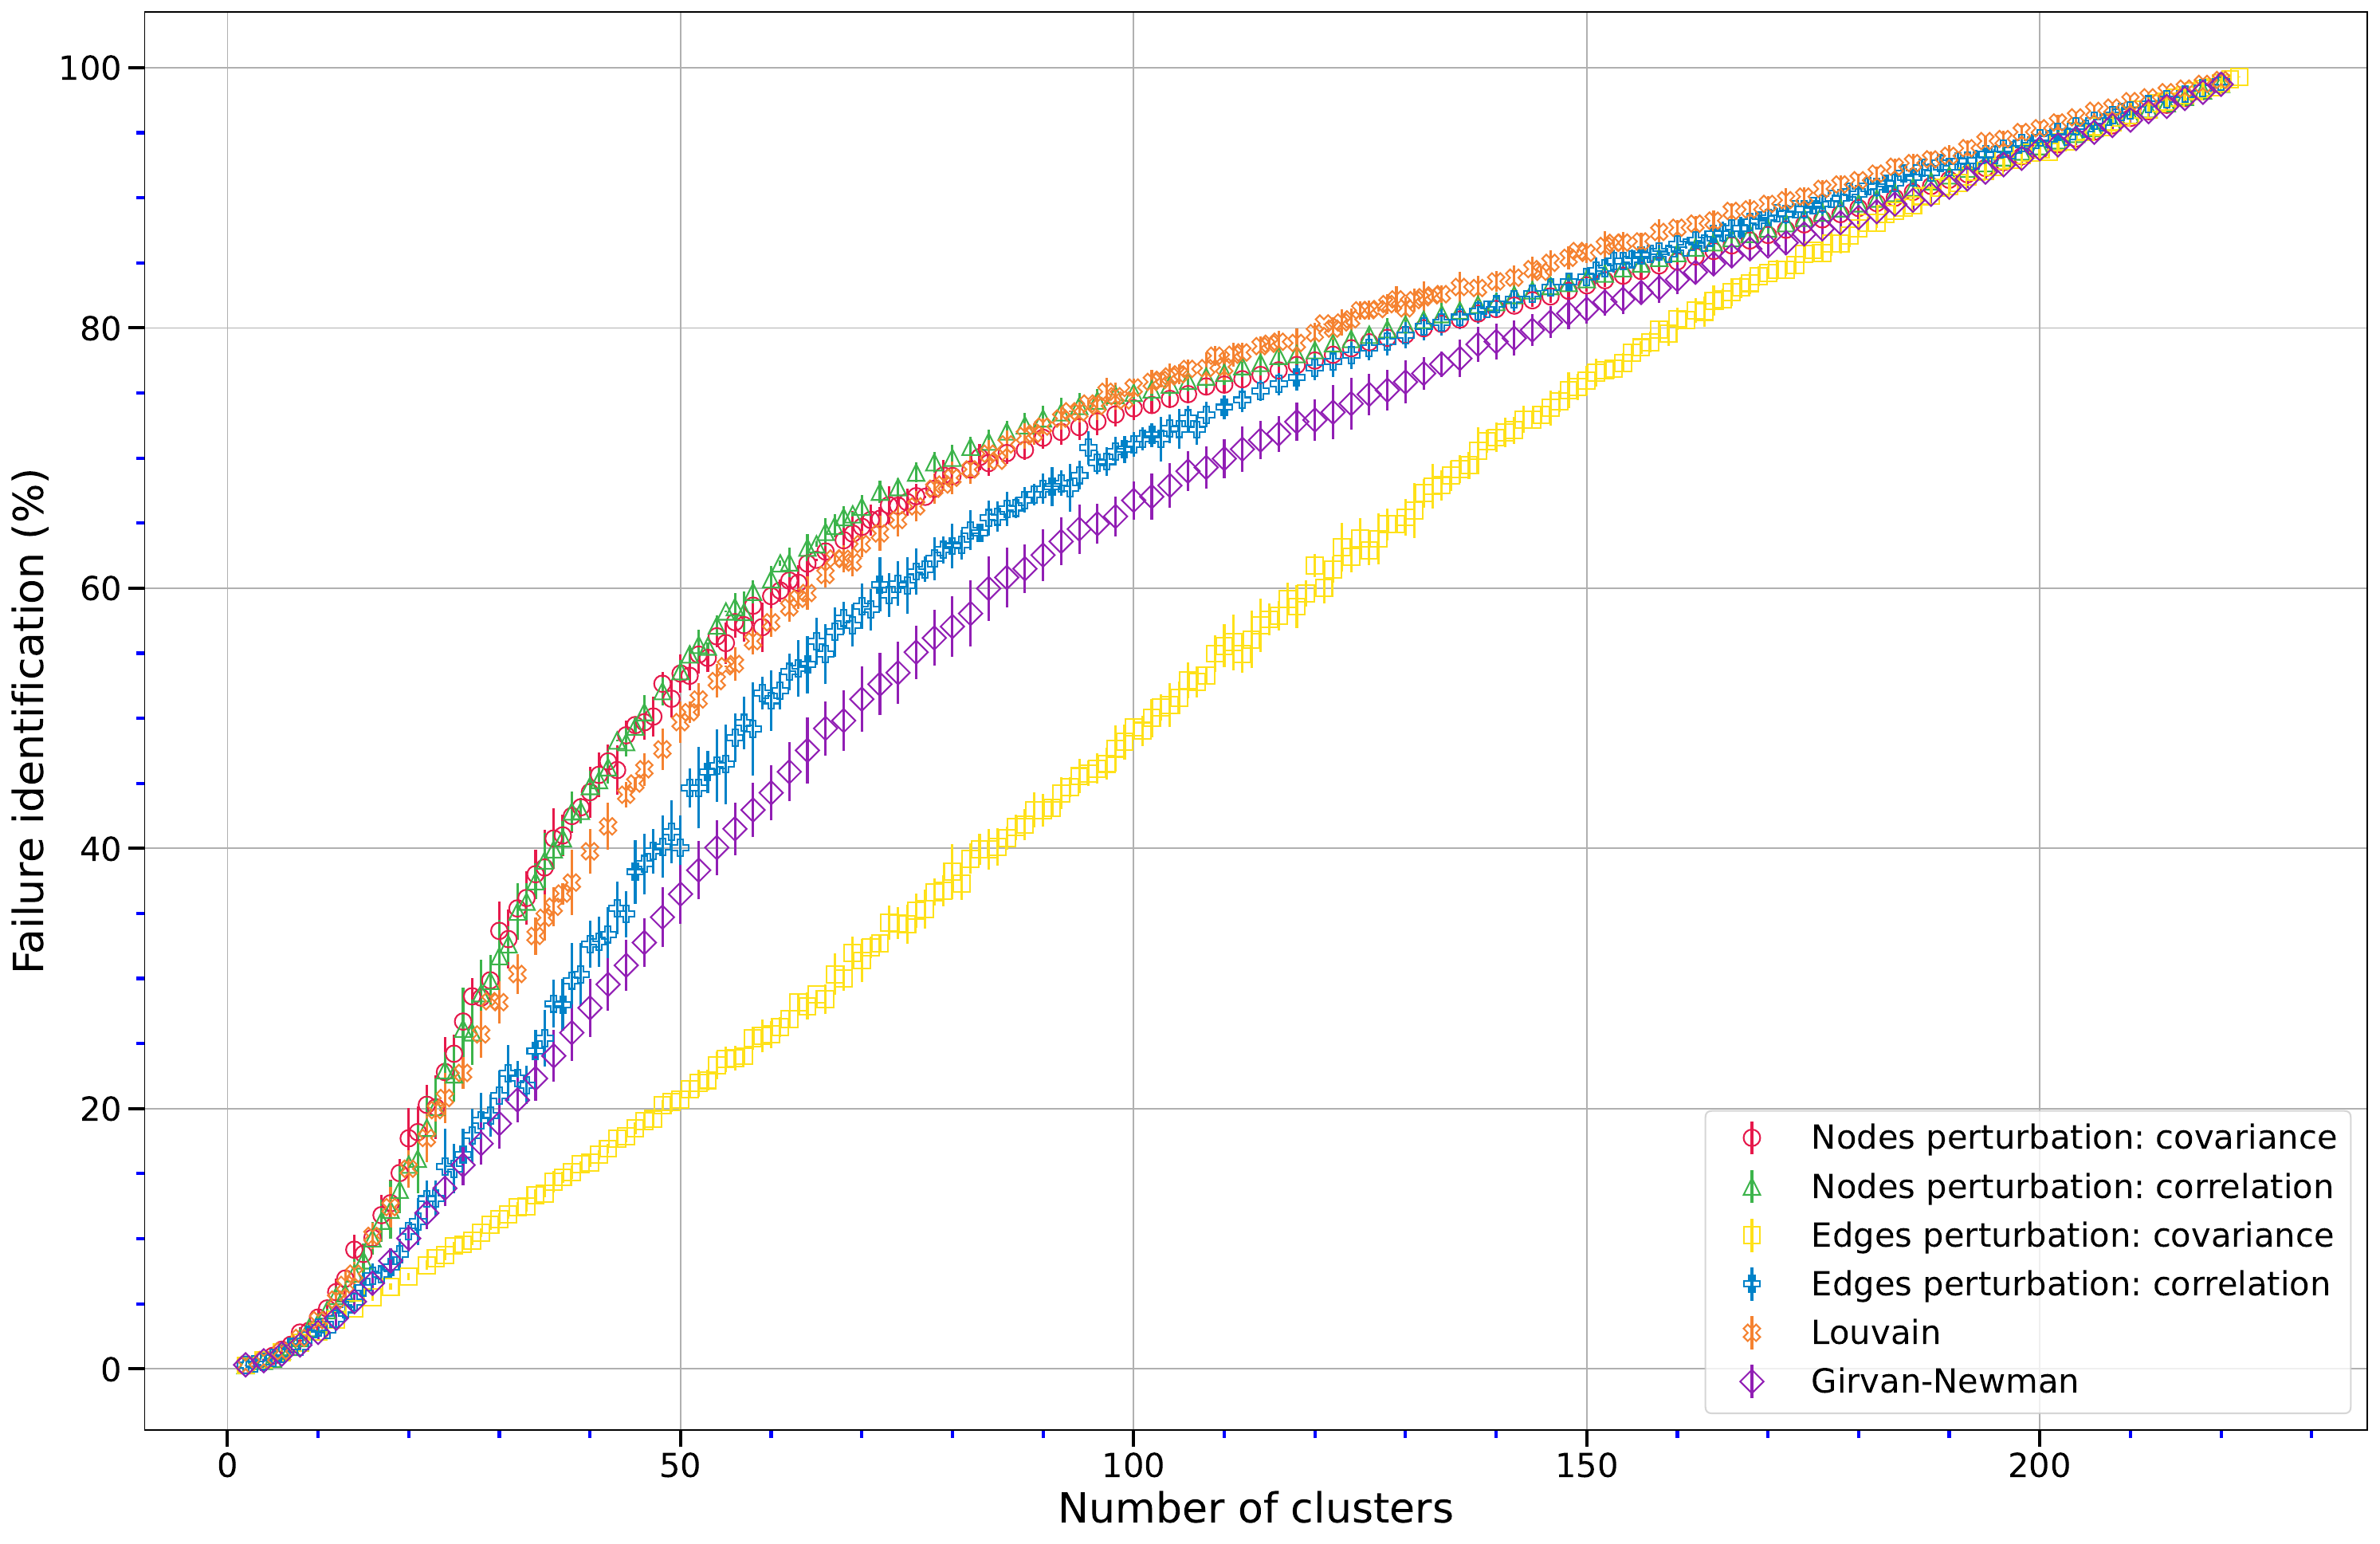}}
\end{figure*}
\begin{figure*}[!htb]
    {\centering
    \includegraphics[width=0.8\textwidth]{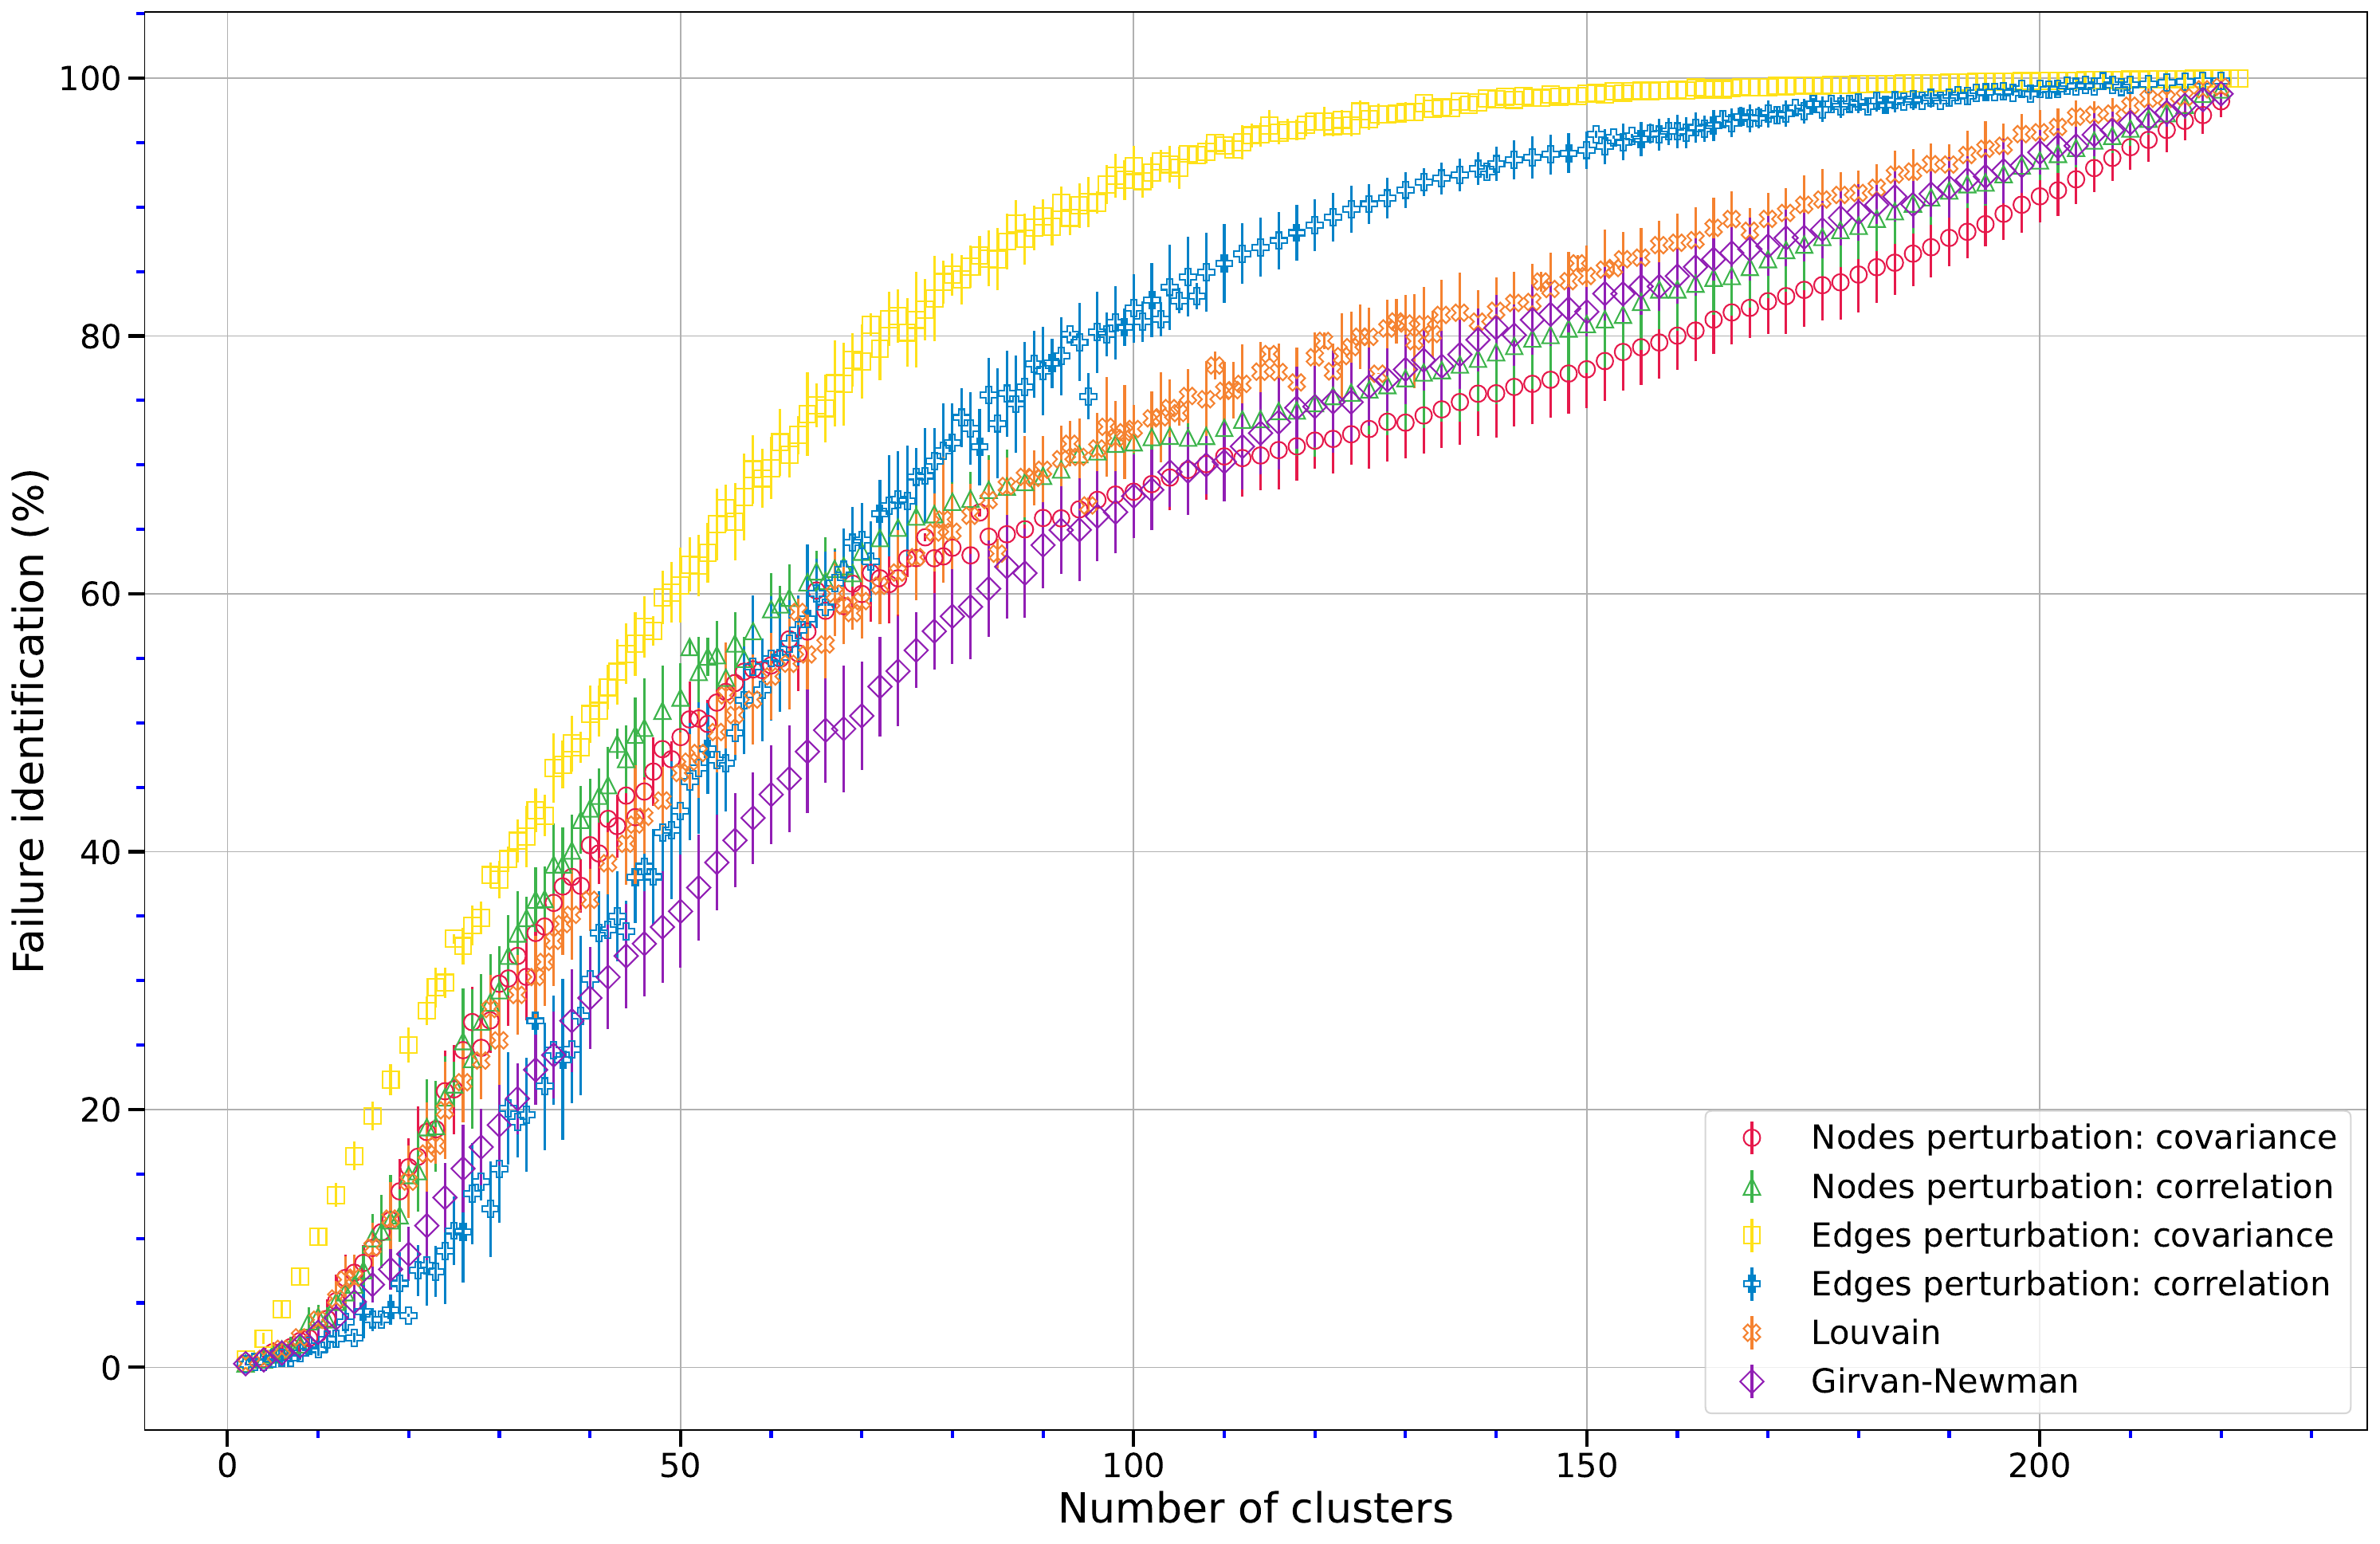}
    \caption{The same numerical results as in Fig. \ref{fig:barabasi-edges} in the case of the 4-Regular random network.}
    }
 \label{fig:regular_edges}    
\end{figure*}

\begin{figure*}[!htb]
    {\centering
    \includegraphics[width=0.8\textwidth]{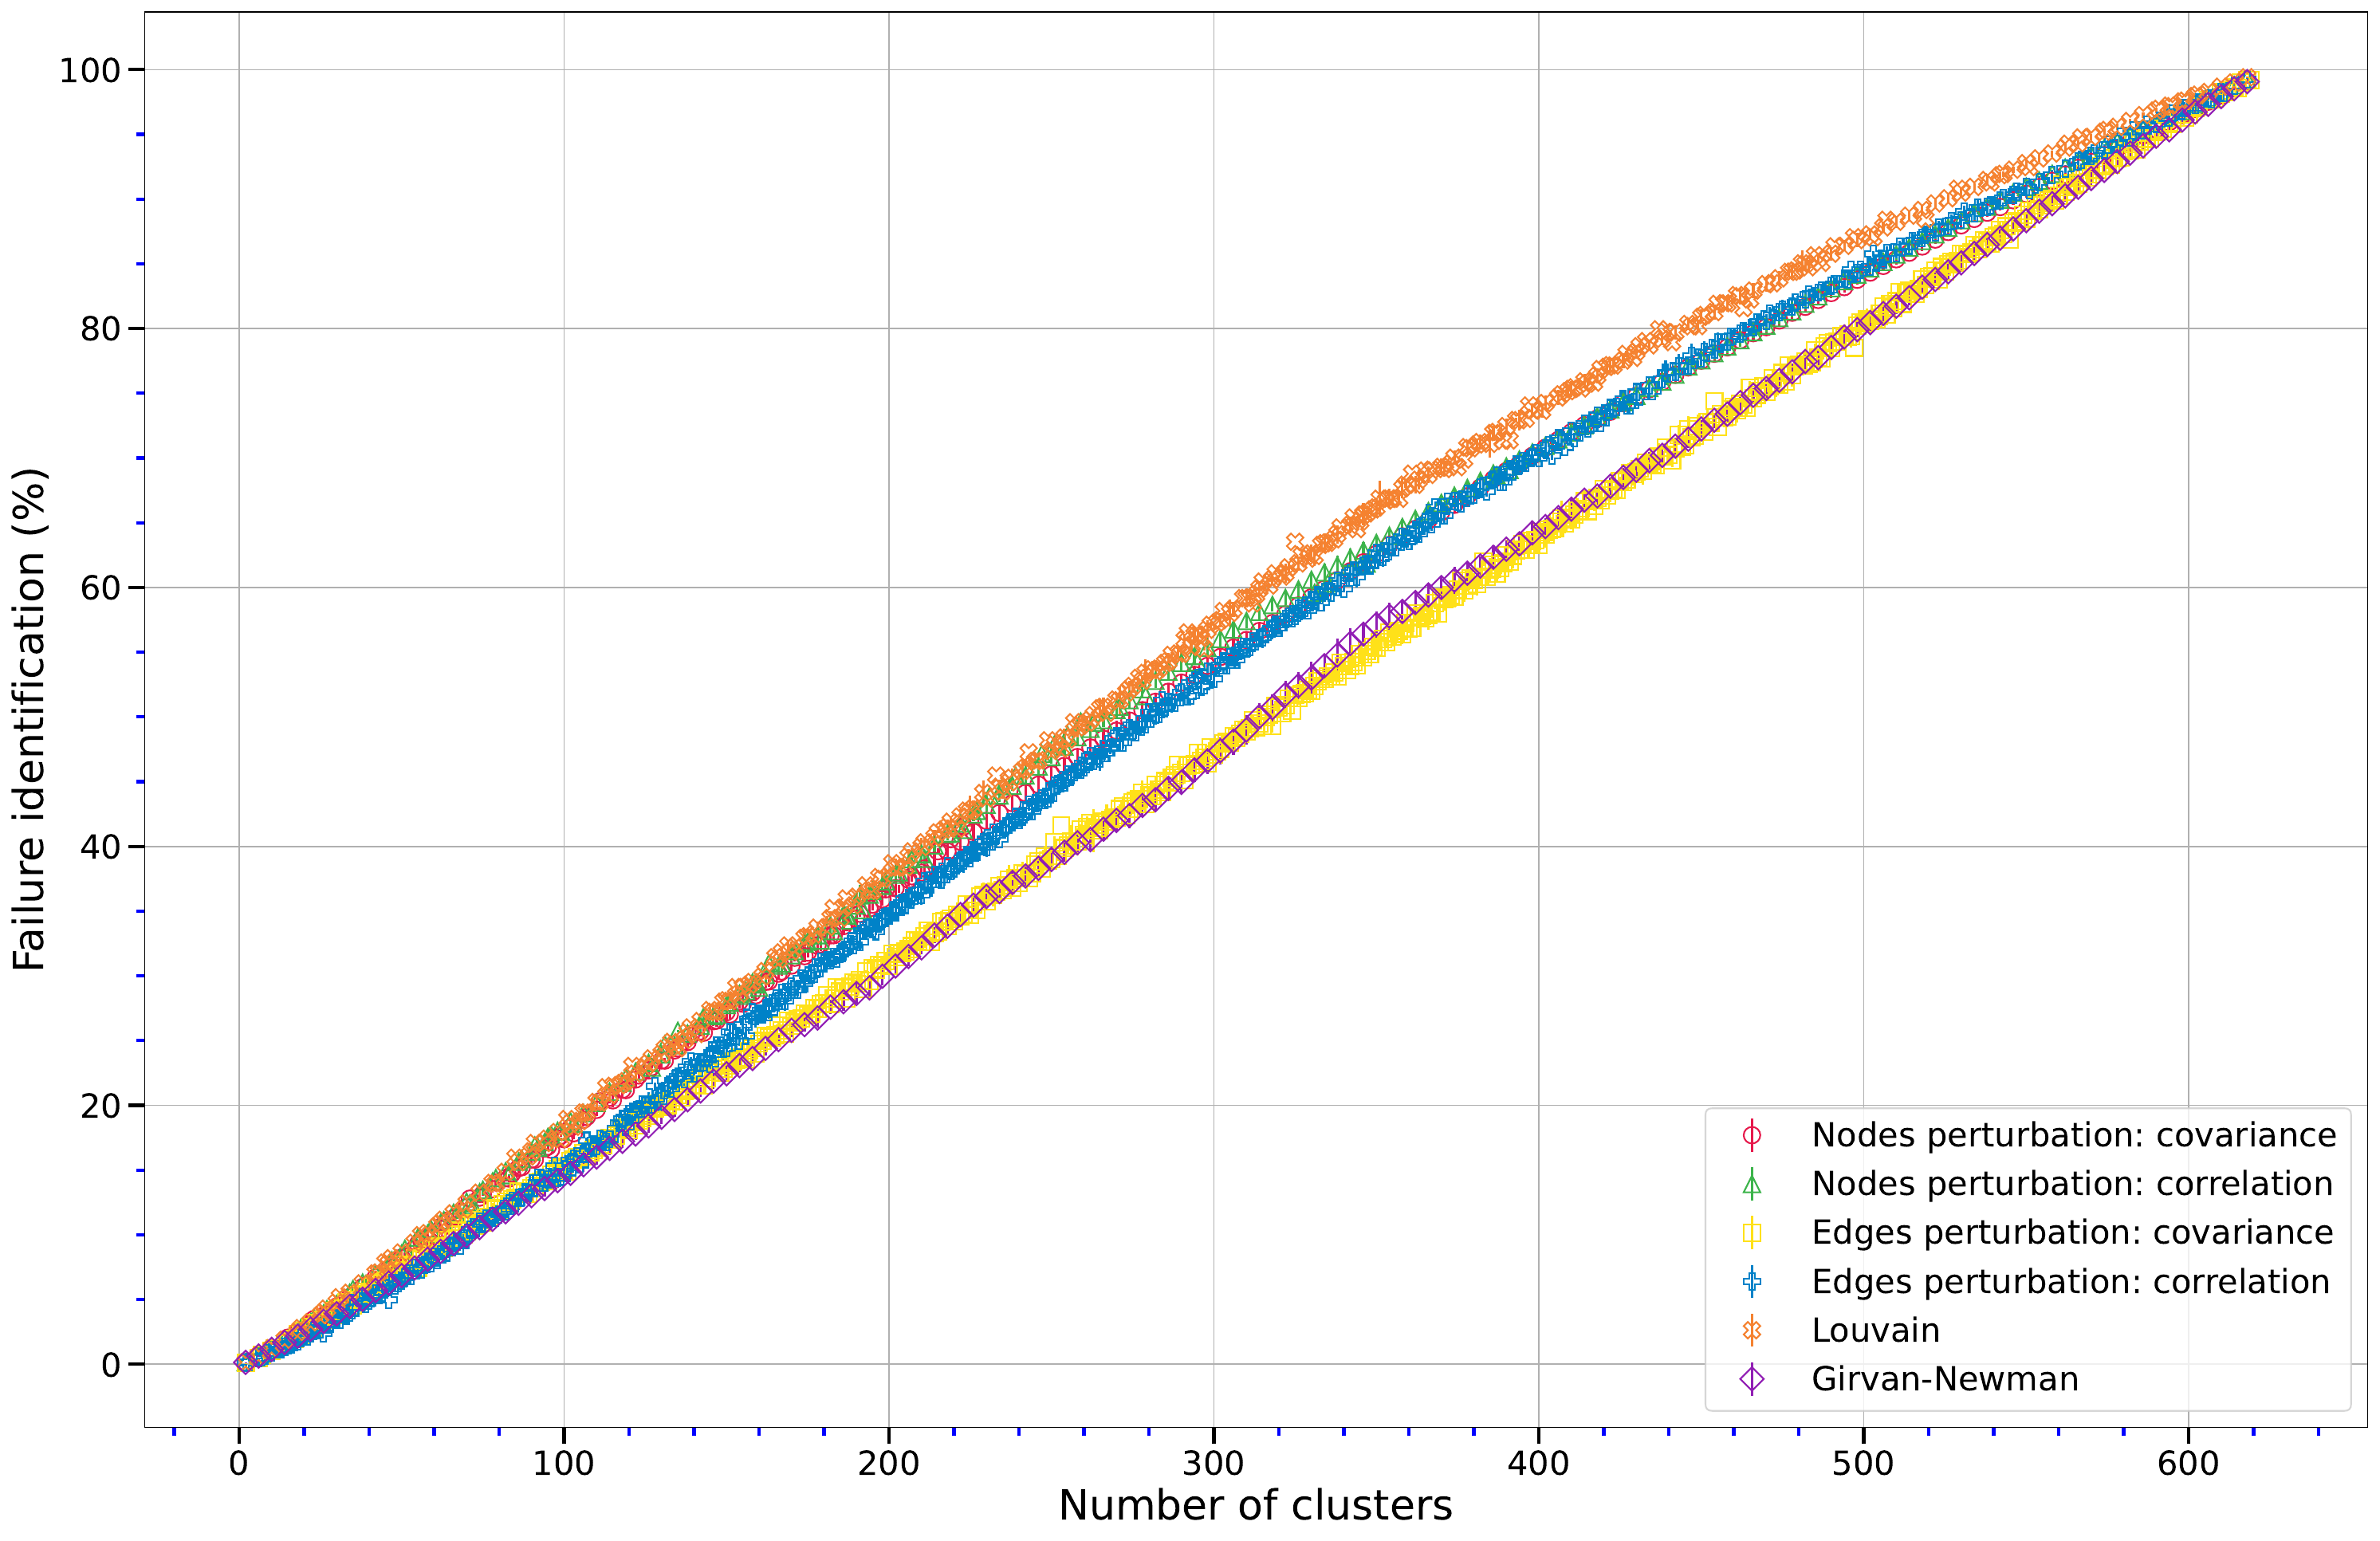}}
\end{figure*}
\begin{figure*}[!htb]
    {\centering
    \includegraphics[width=0.8\textwidth]{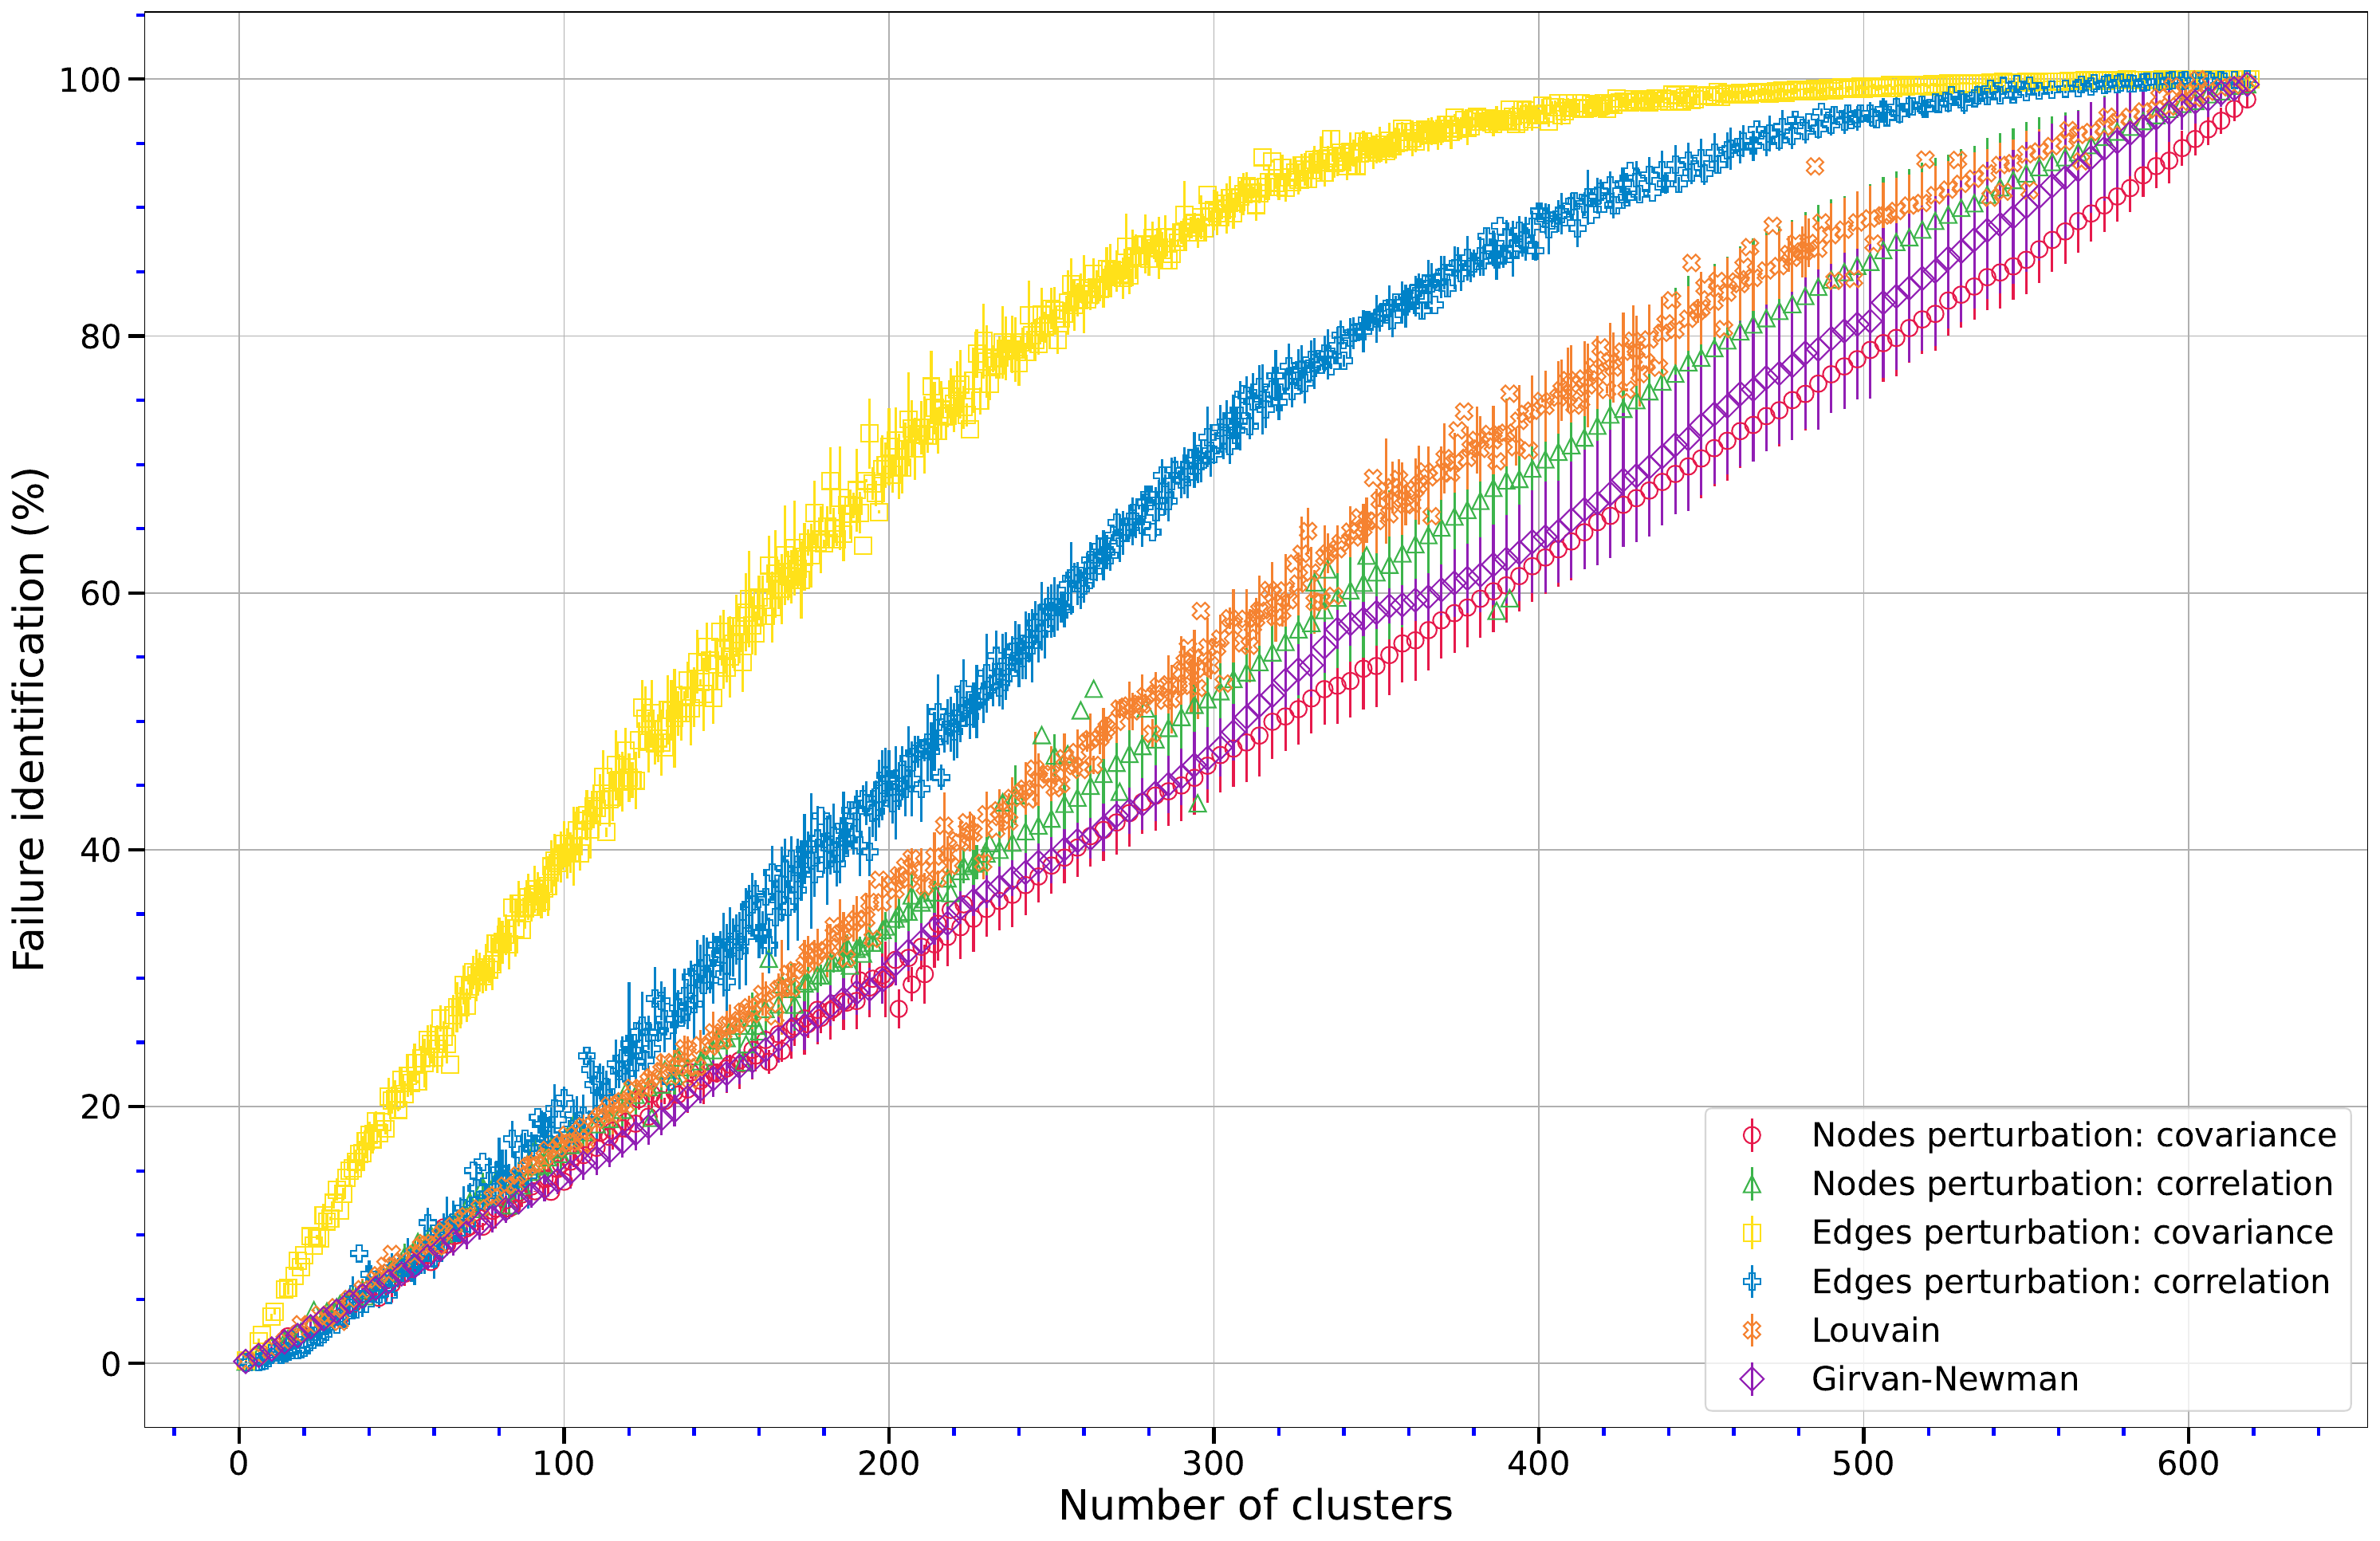}
    \caption{\textcolor{red}{Failure detection efficiency for a grid network of size $25\times 25$ ($625$ nodes). There are no discernible differences between these results and Figure 5 in the main text, despite the number of nodes being almost three times higher. The same higher number of nodes was attempted for the Erdős–Rényi random network, yet again resulting in no appreciable differences.}}
    }
 \label{fig:regular_edges}    
\end{figure*}

\end{document}
